# Supplementary material for: Cell Model Approaches for Predicting the Swelling and Mechanical Properties of Polyelectrolyte Gels
Source: arXiv:1908.10804 source file (2019-11-06)

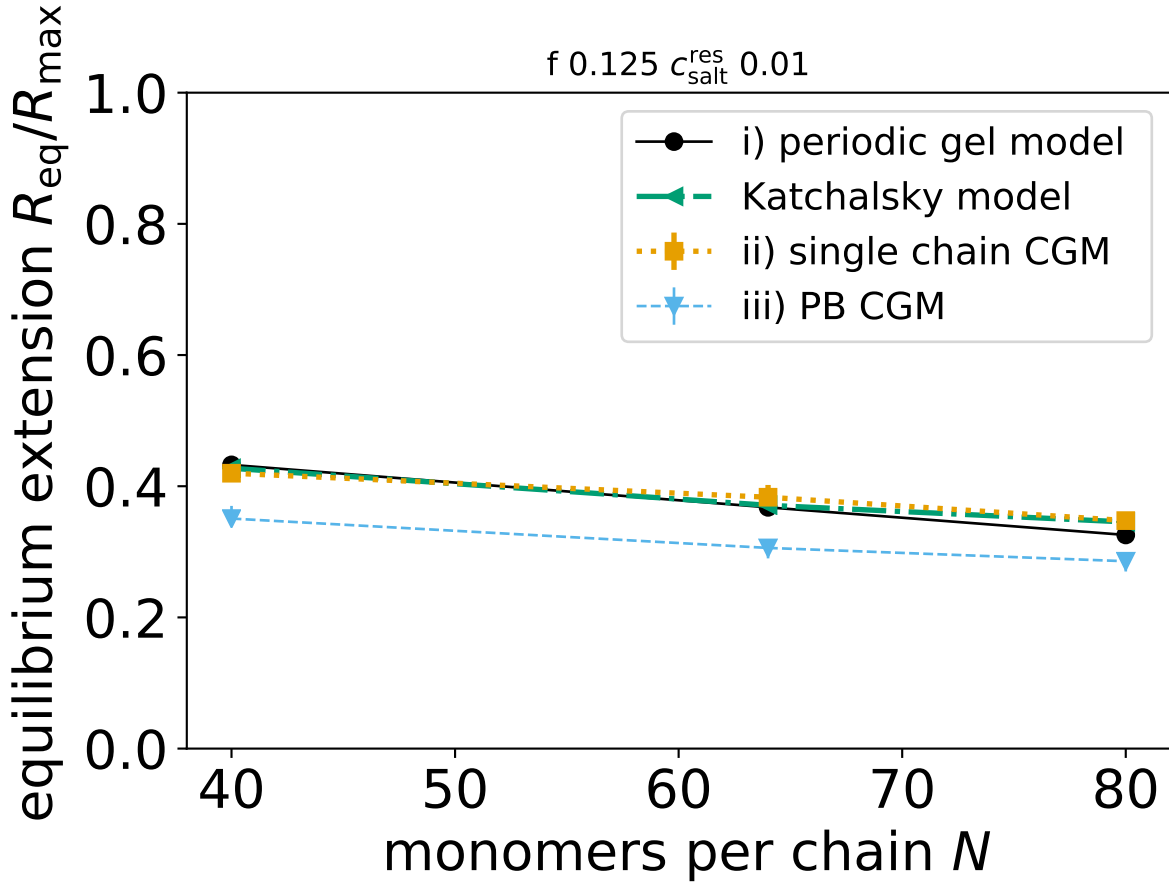

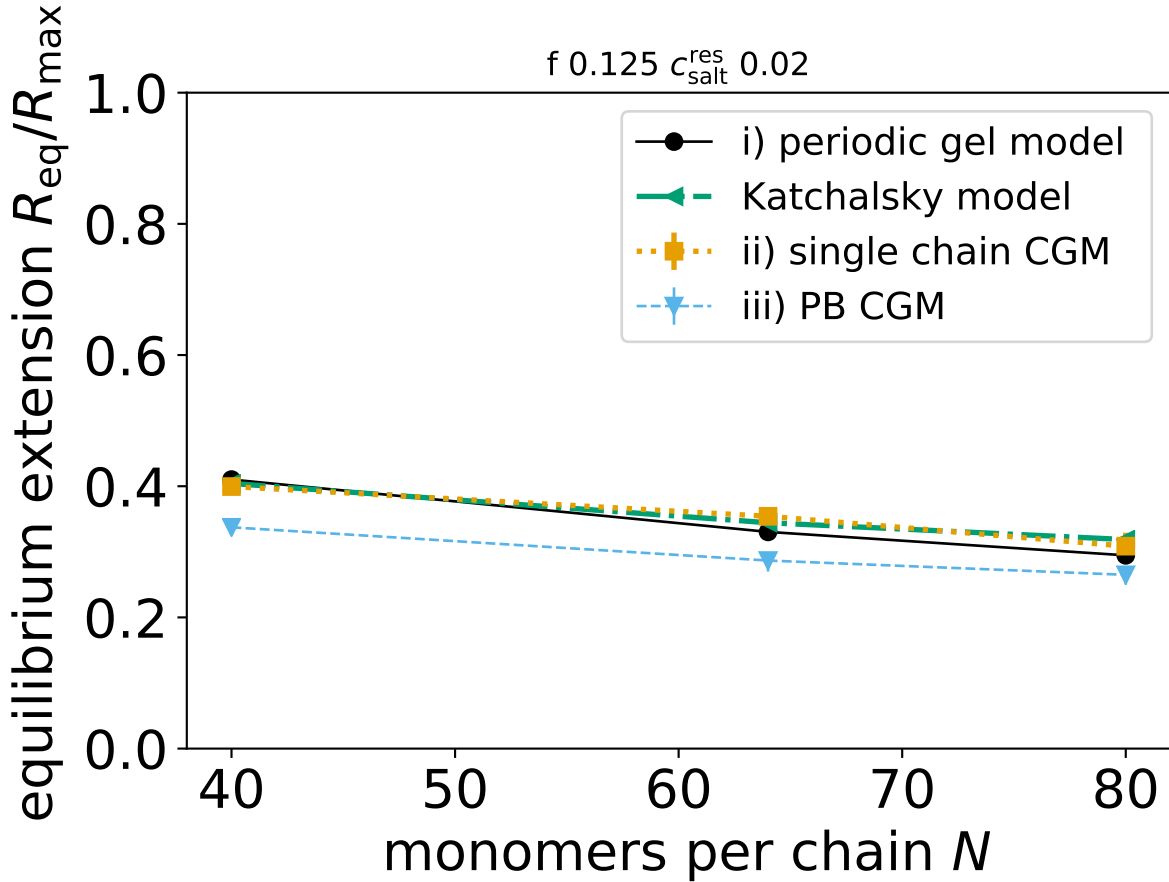

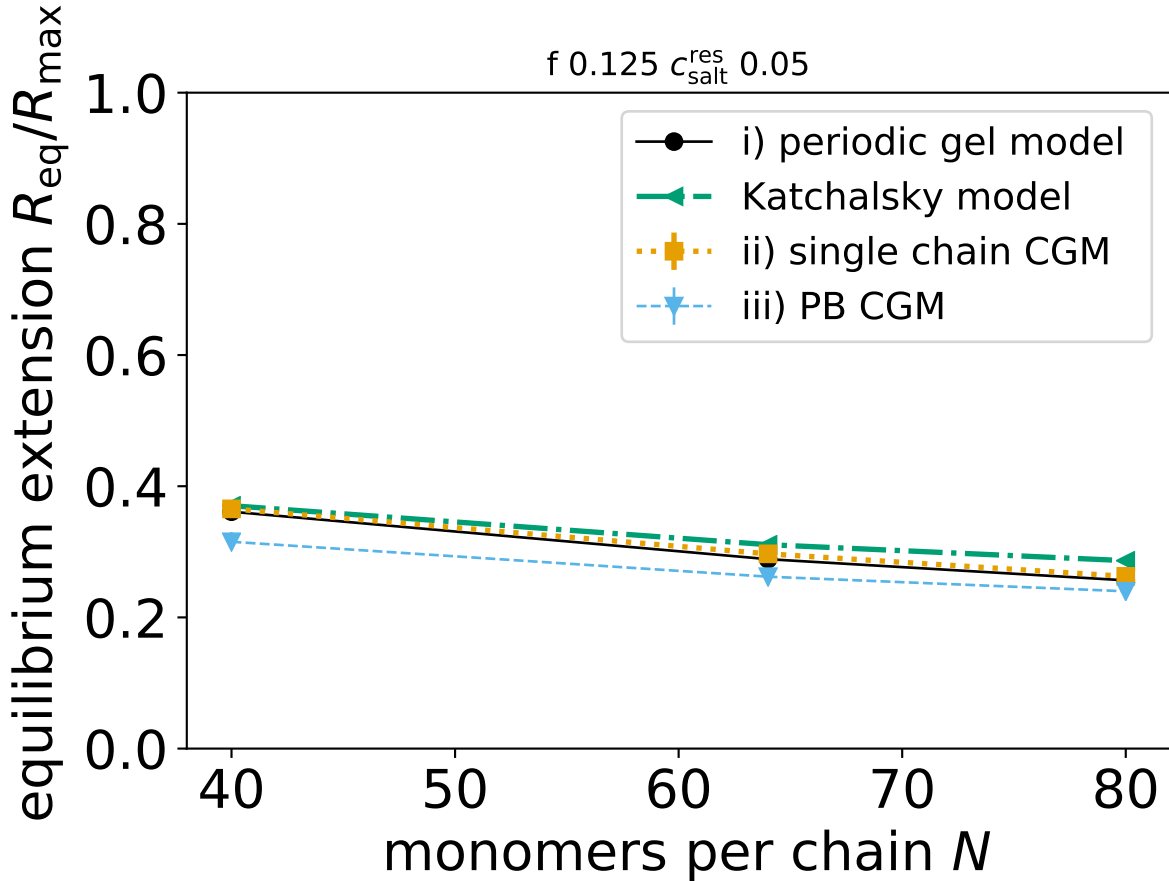

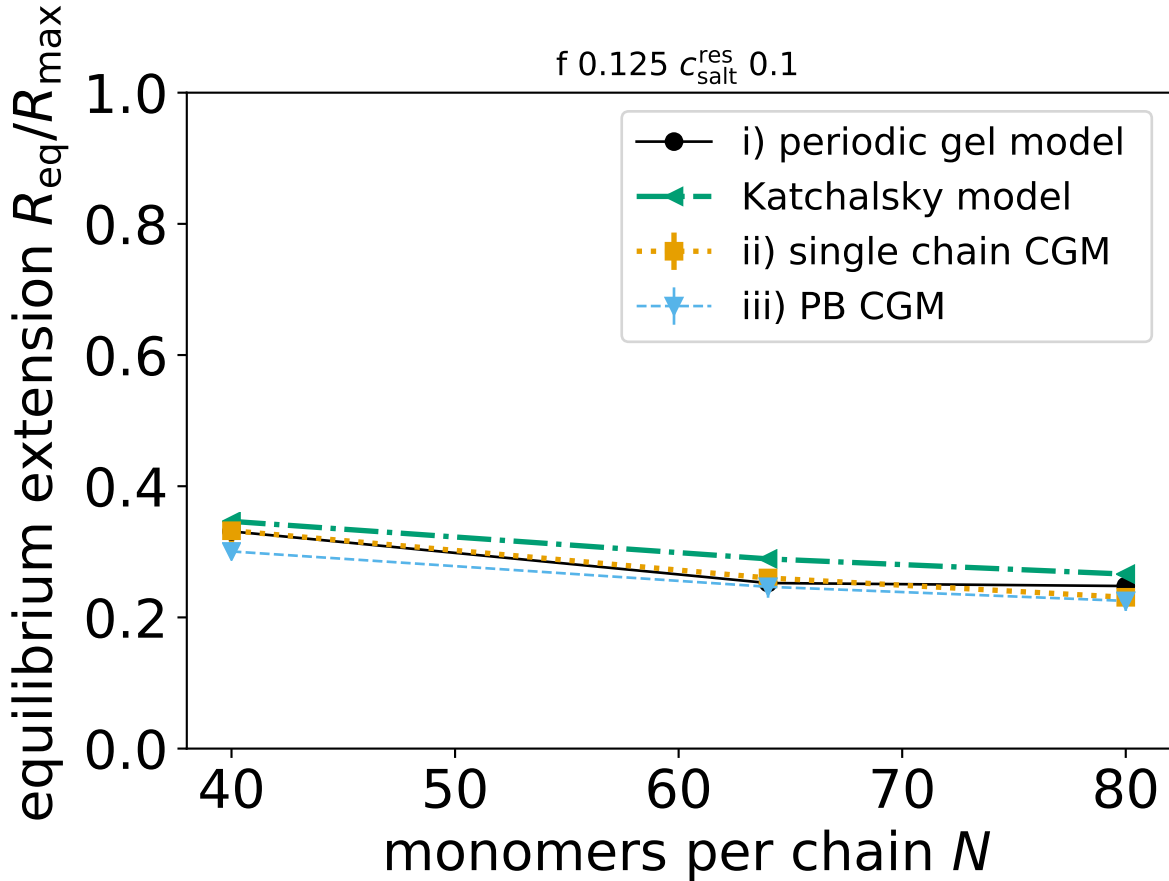

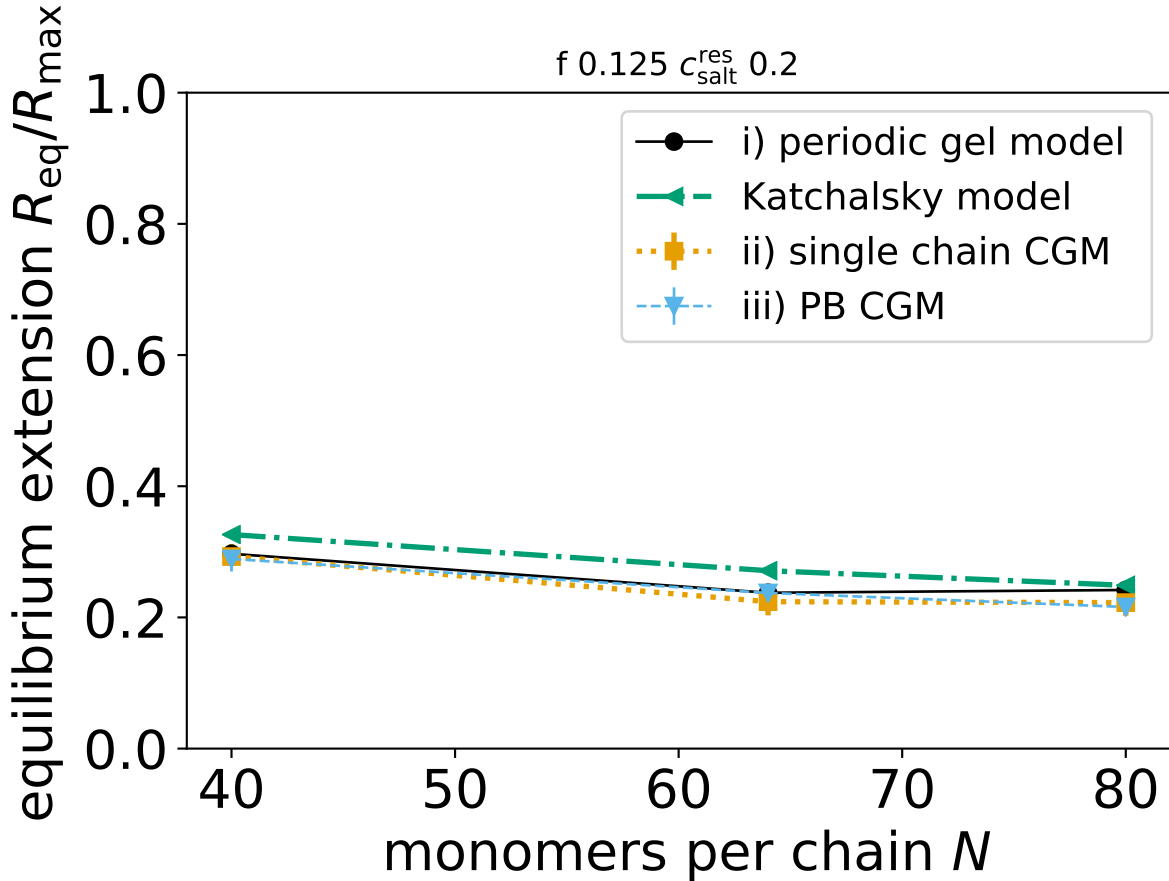

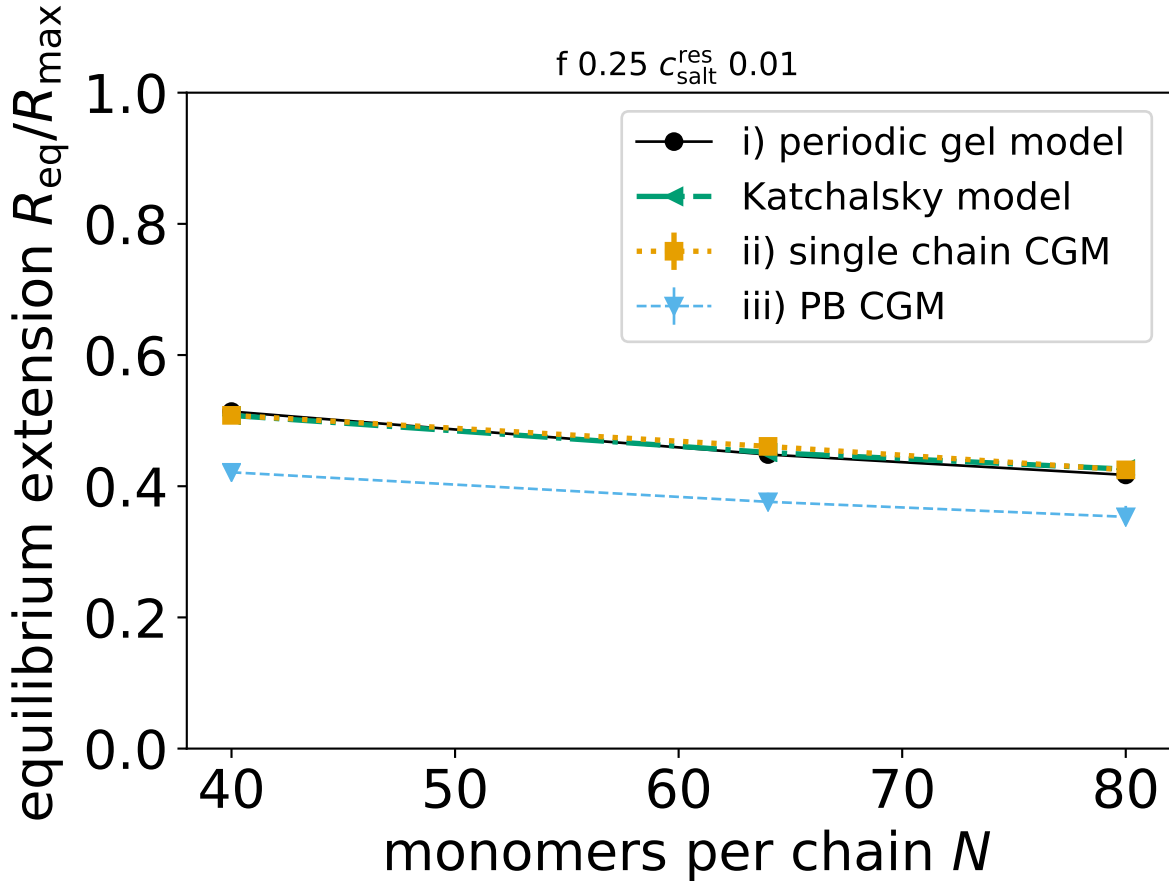

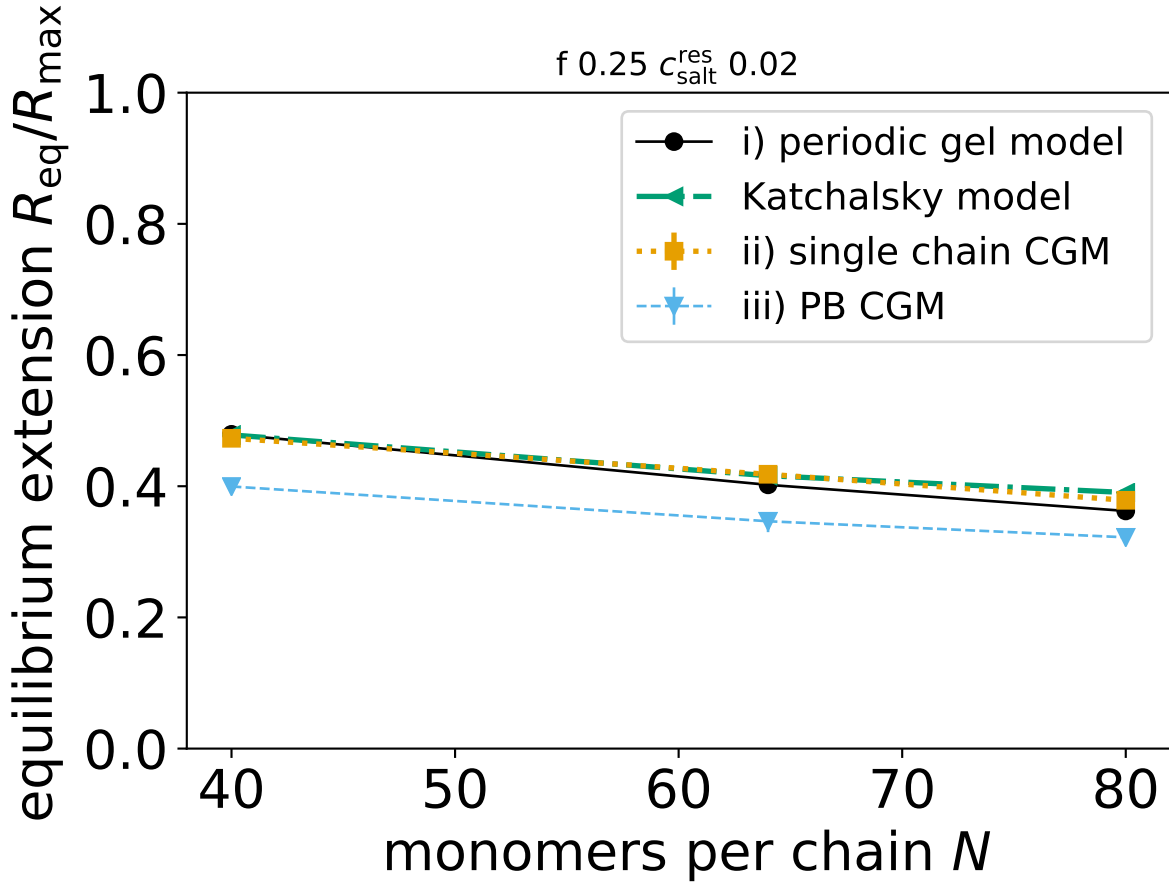

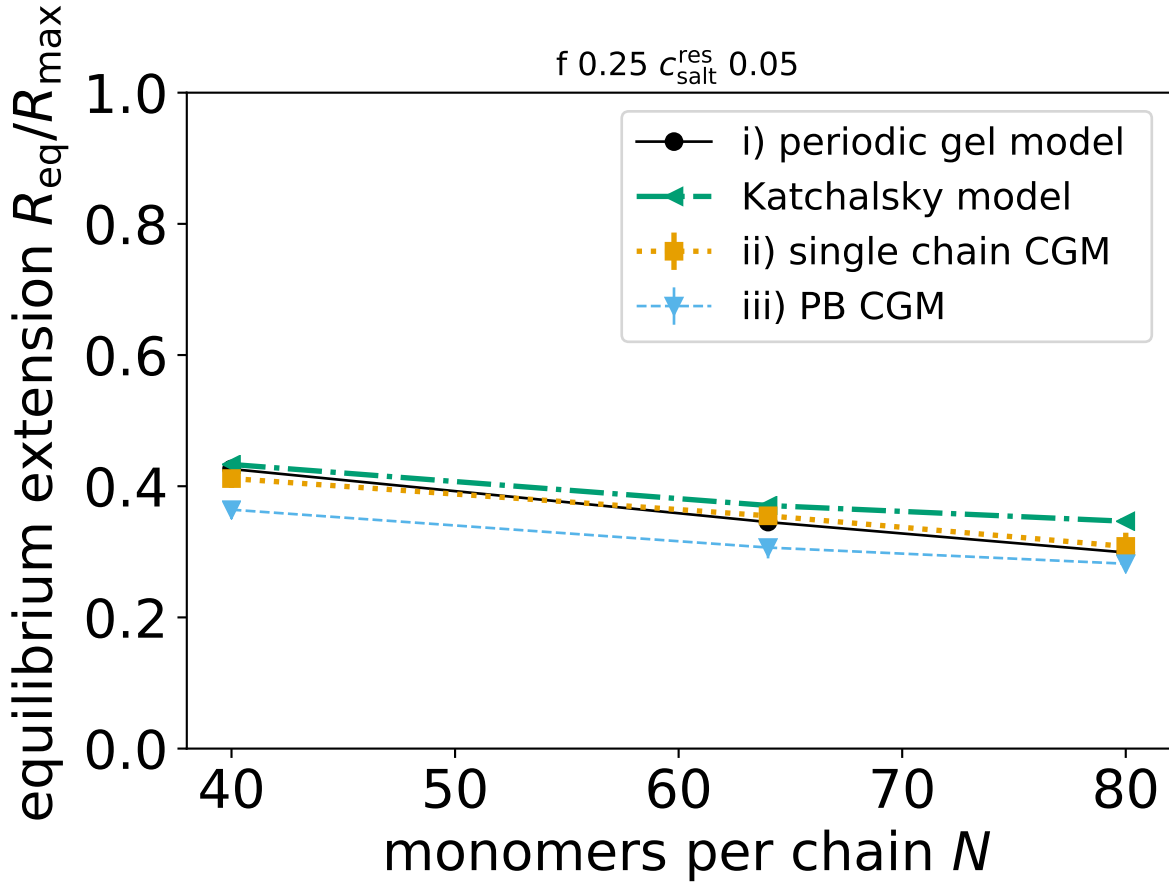



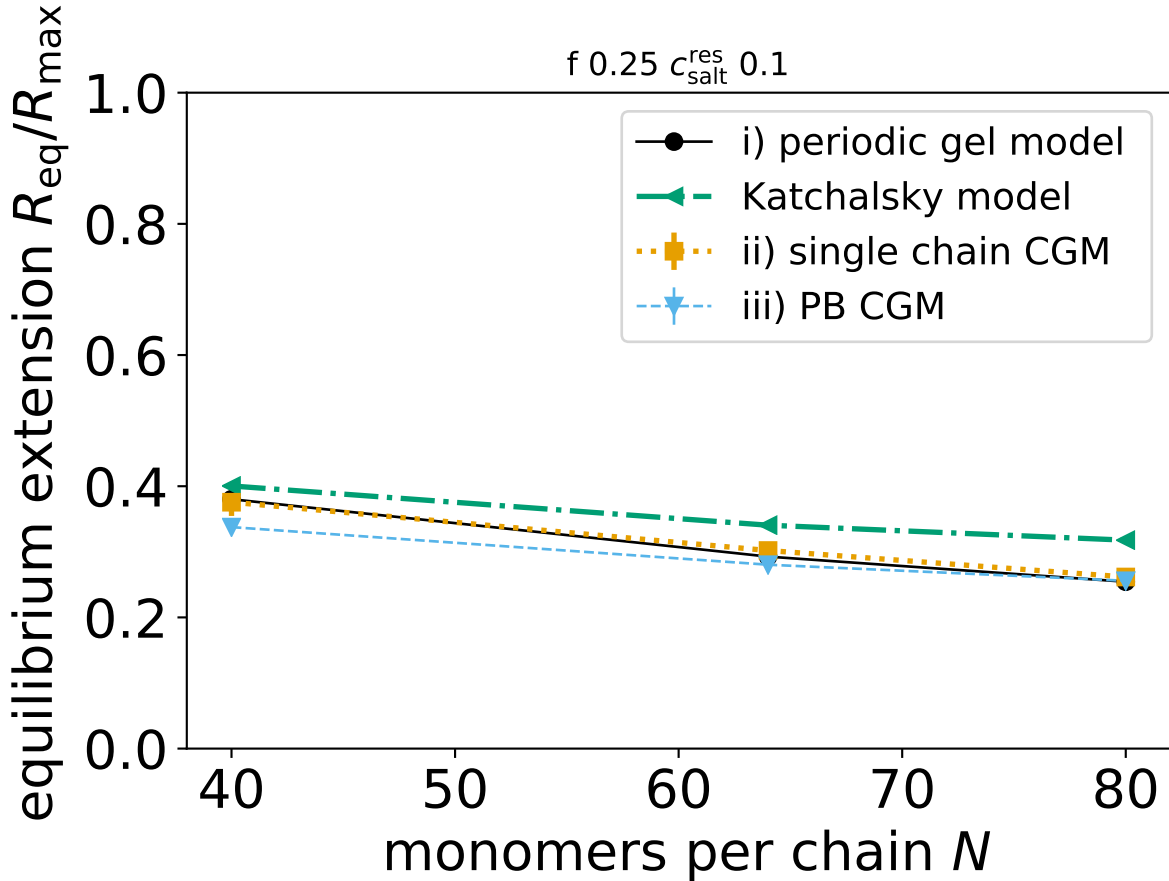

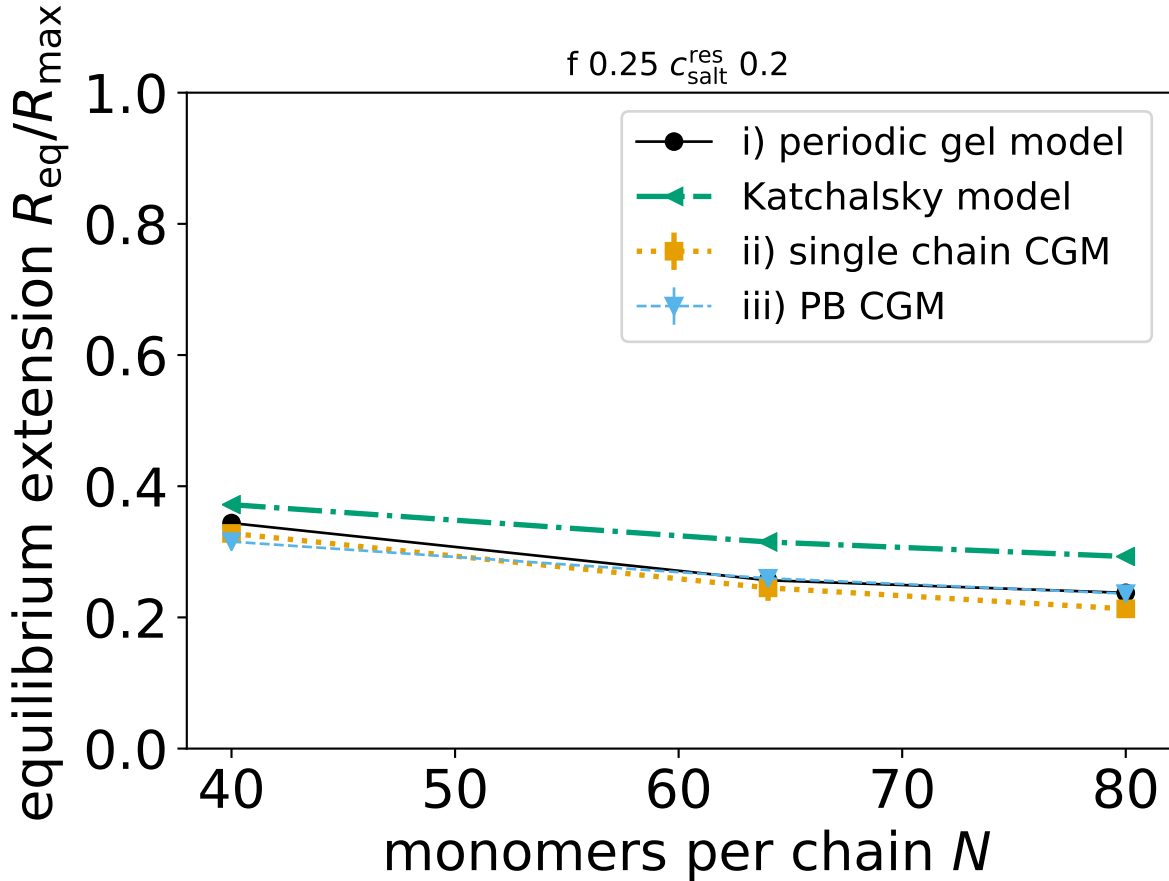

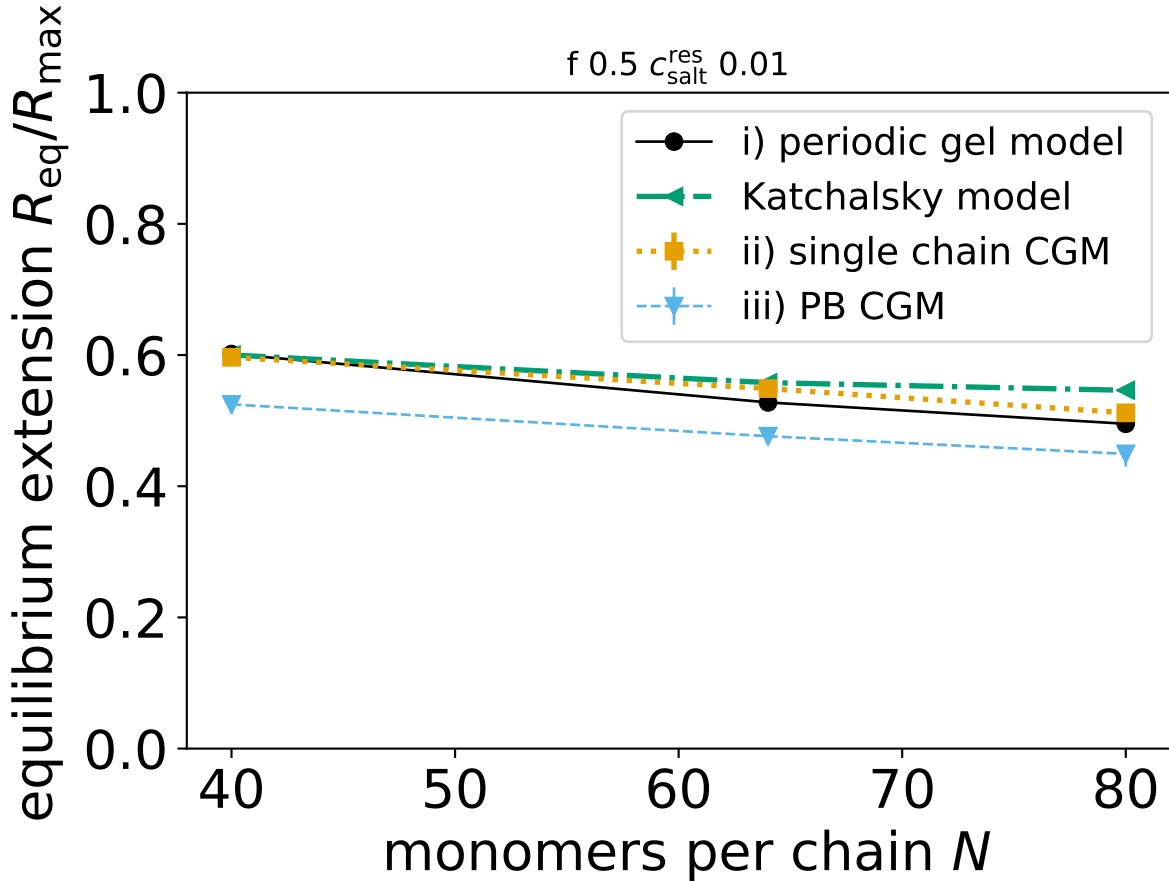

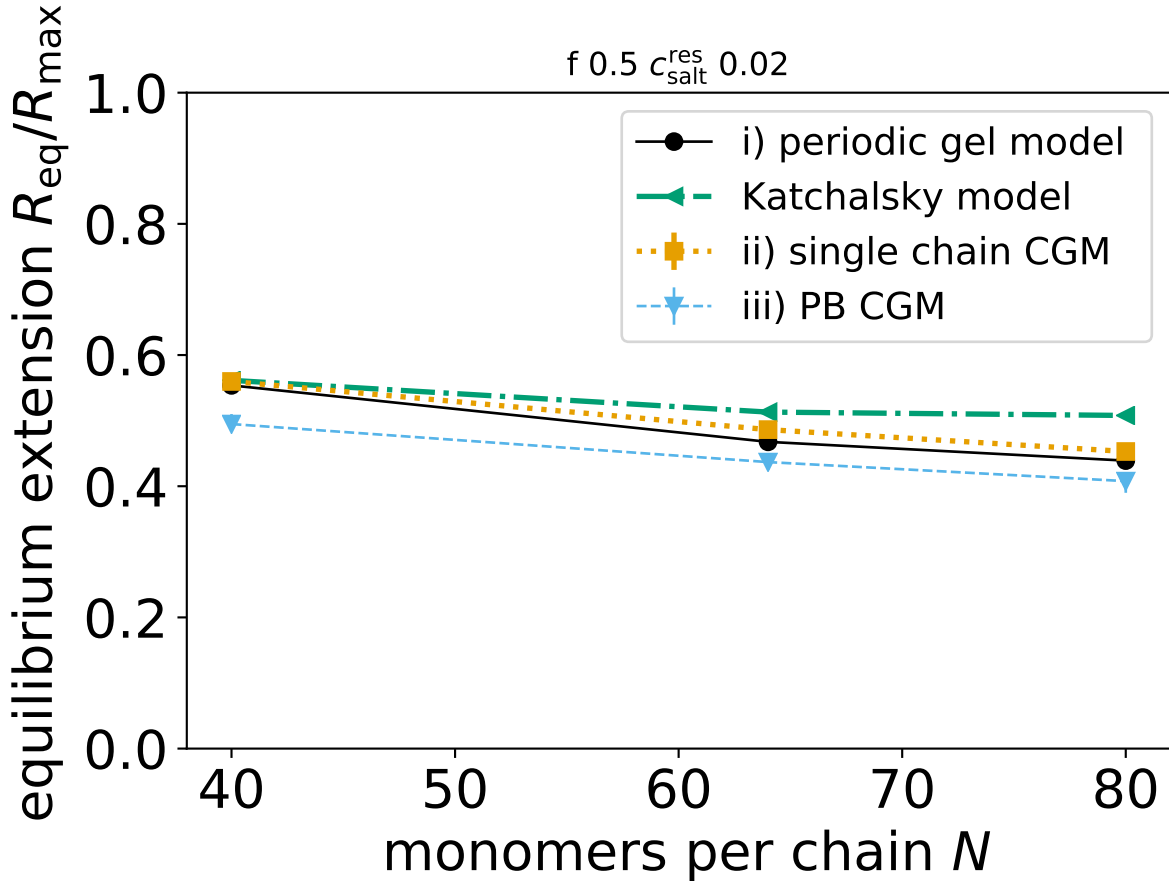

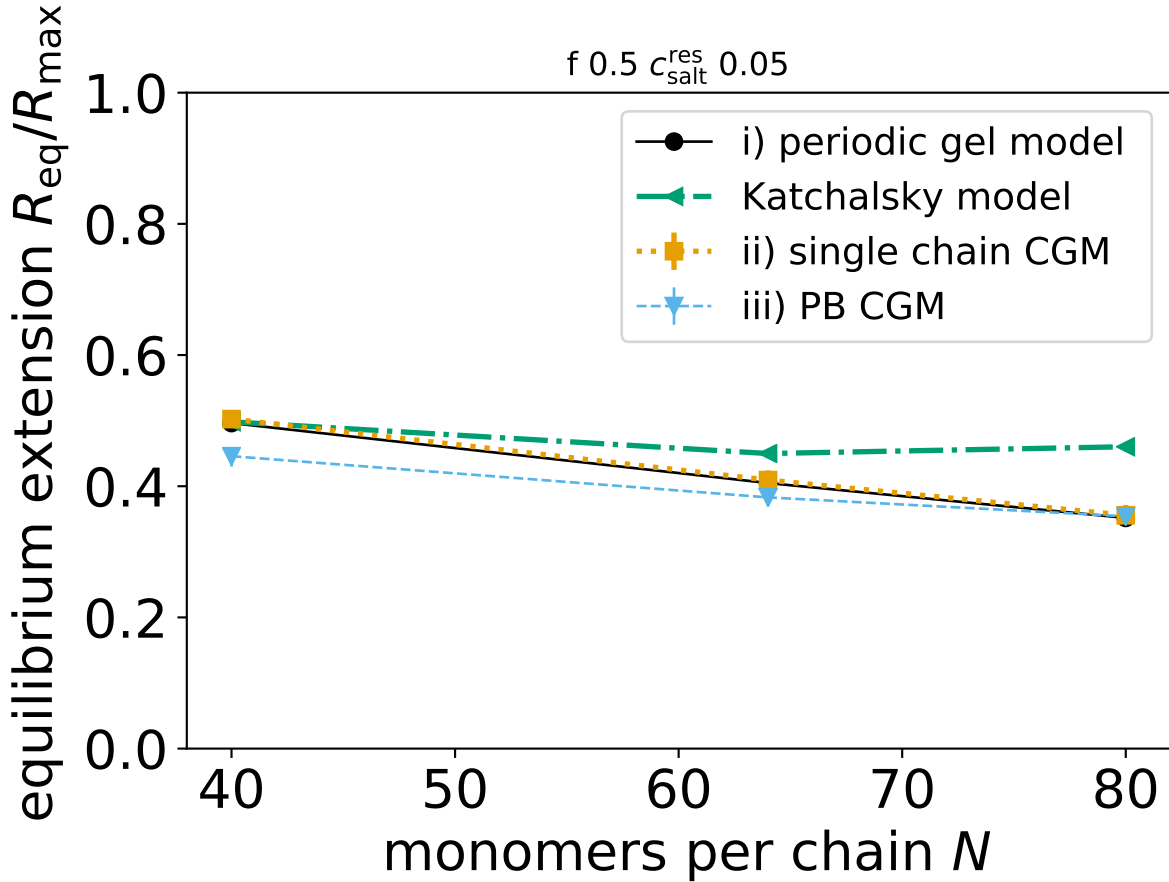

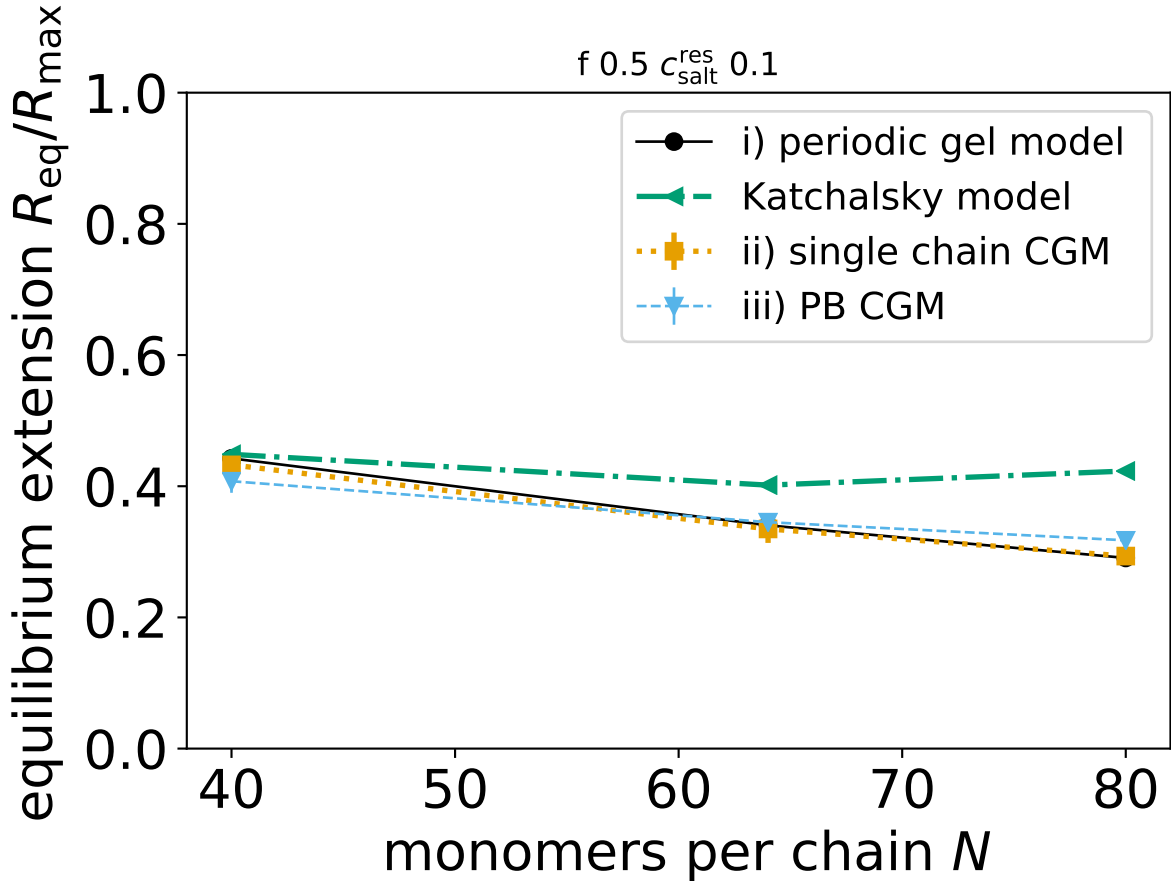

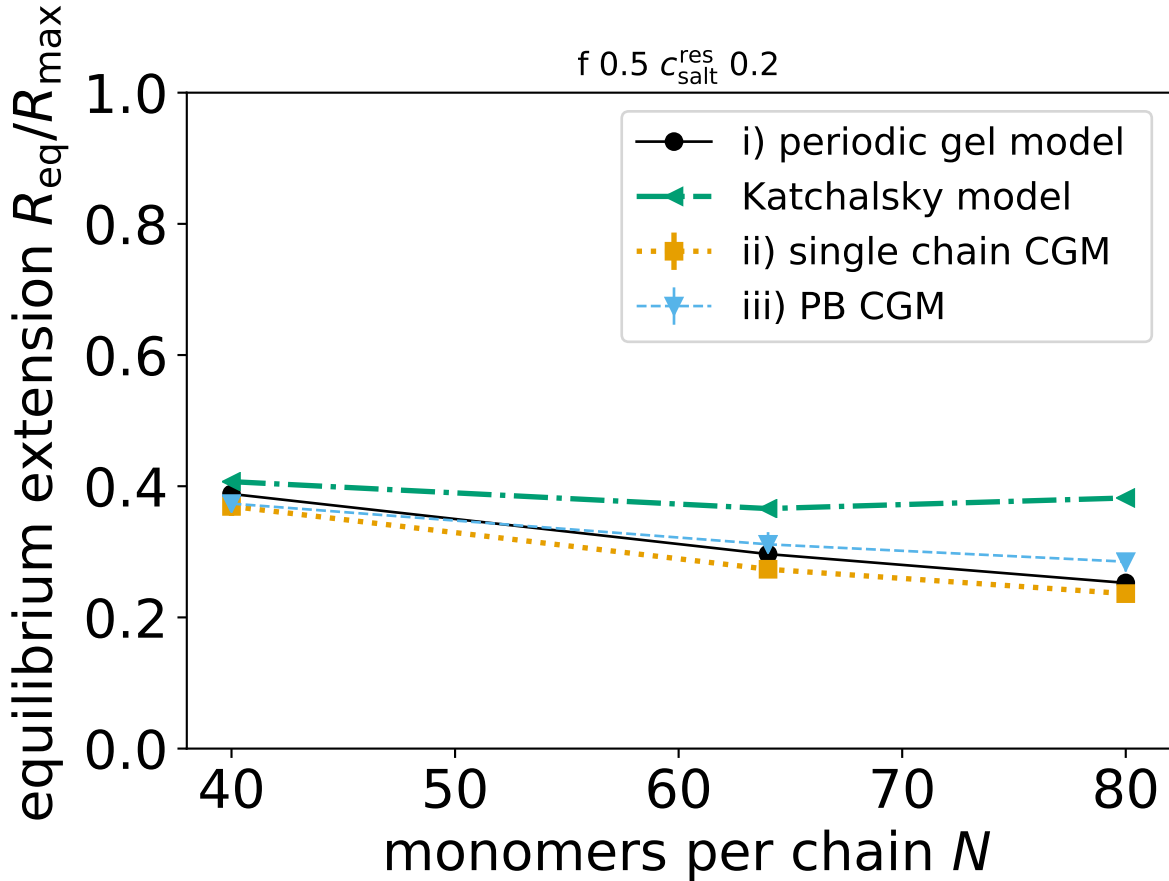

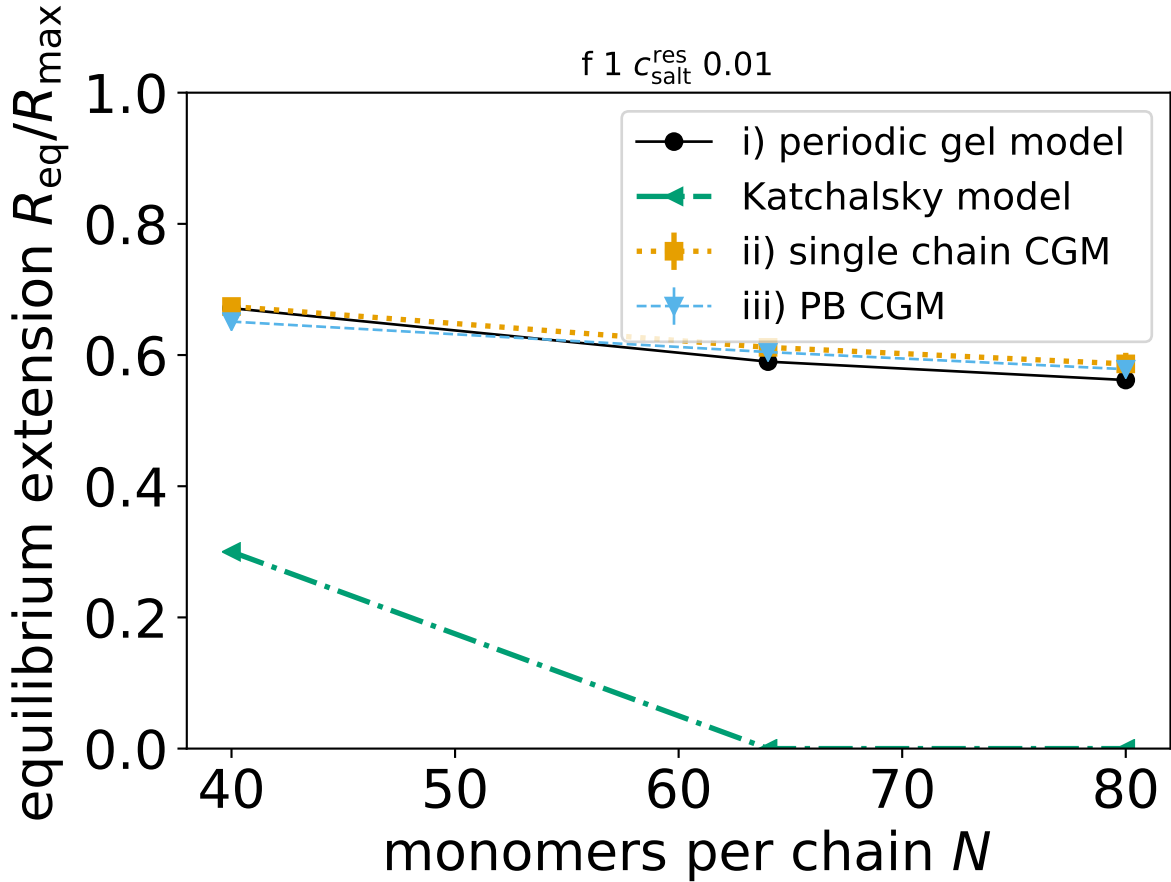



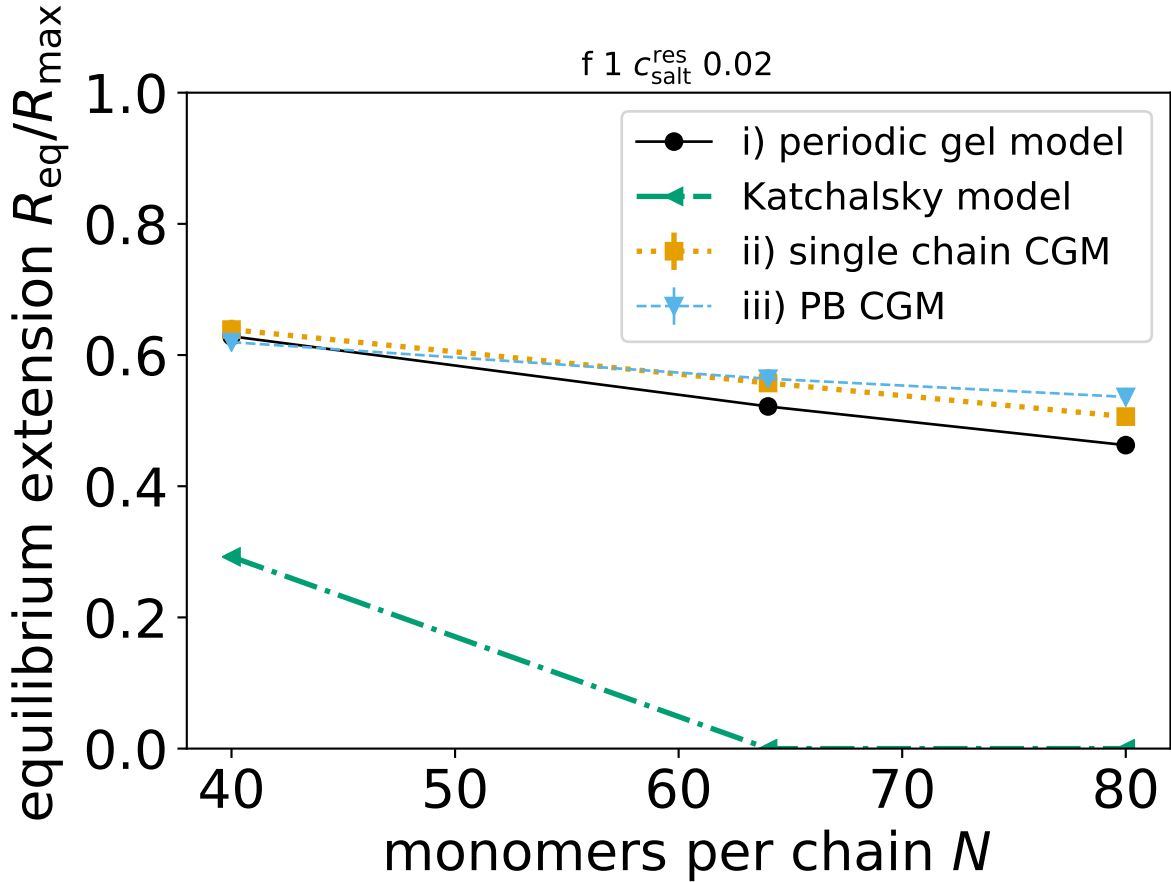

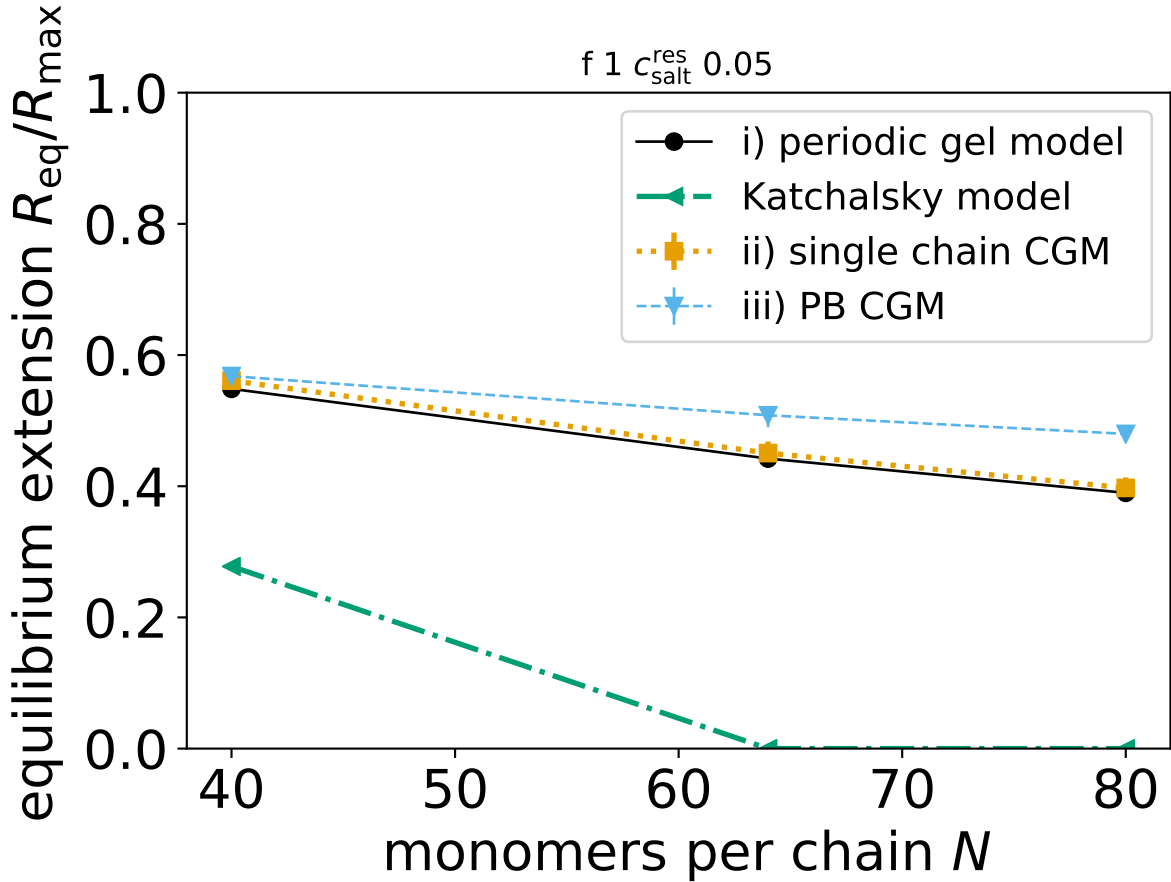

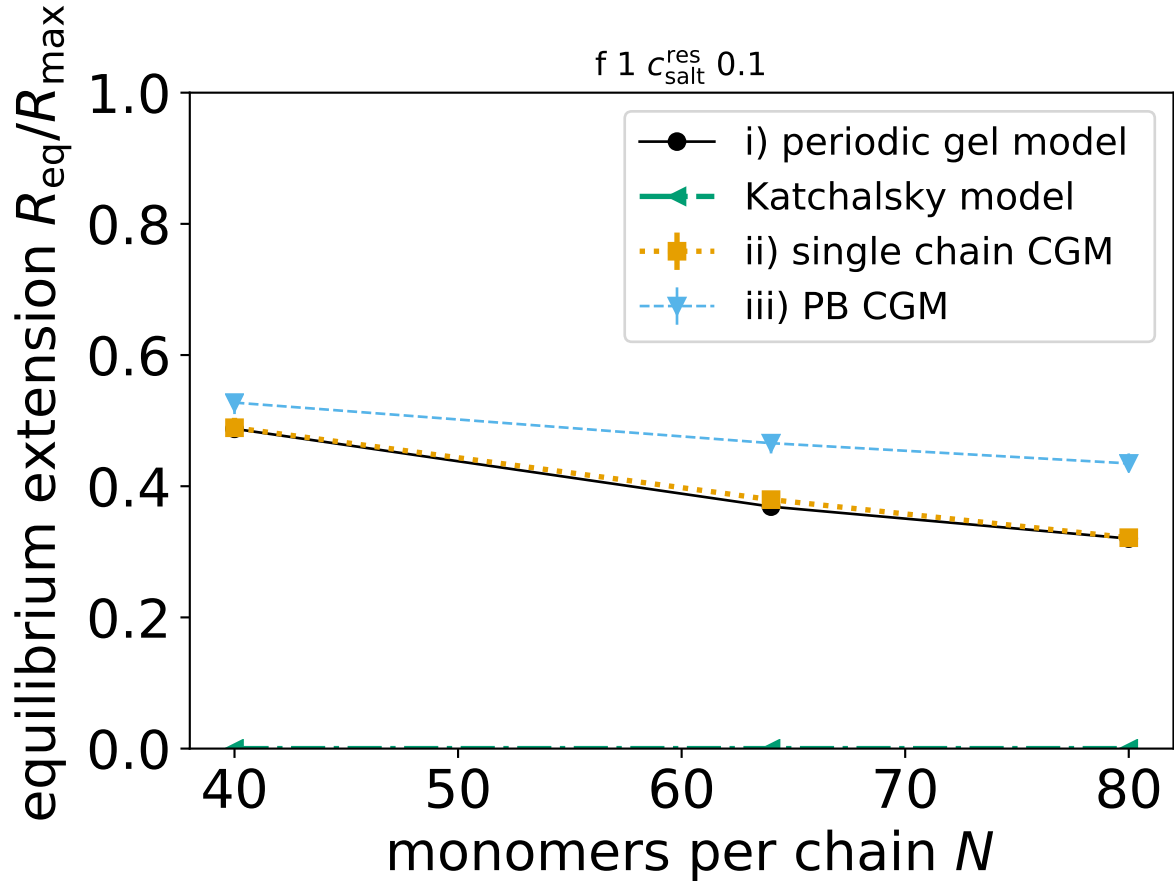

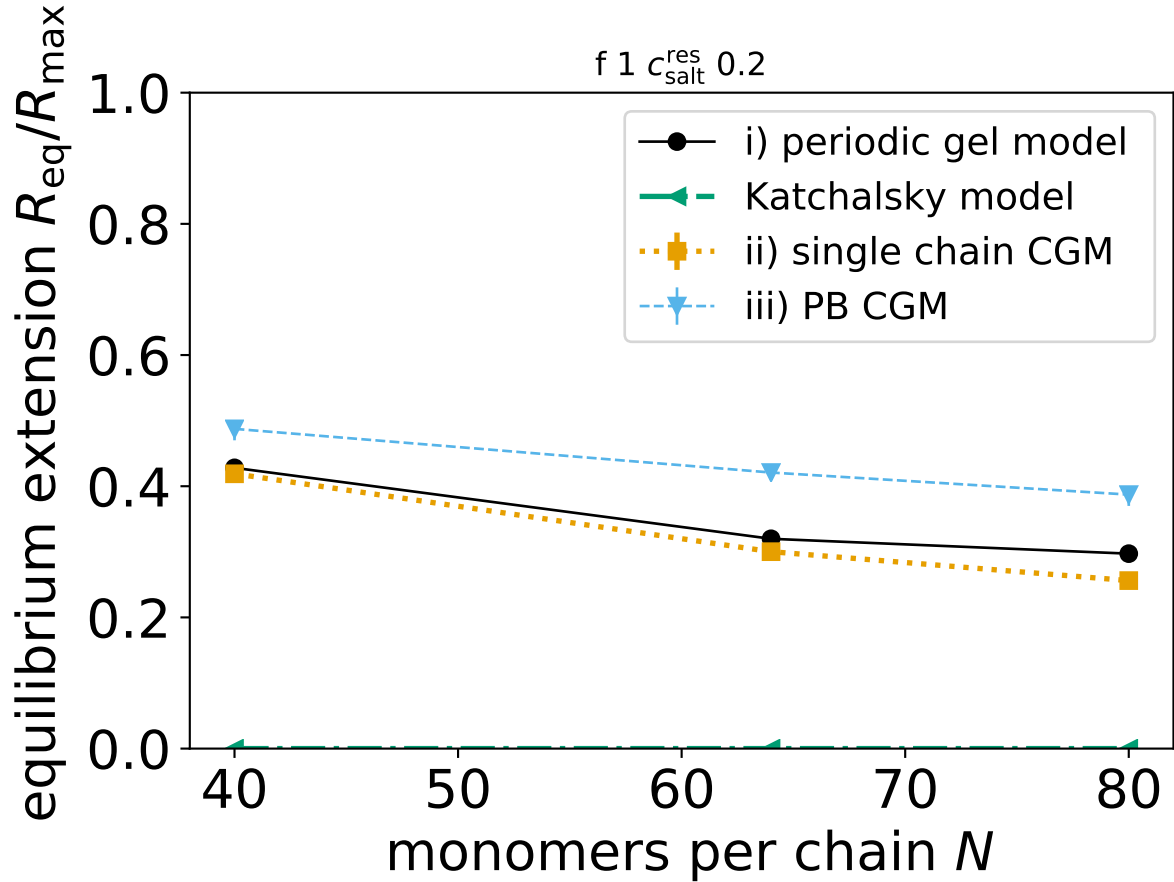

Supplement: Supplementary file 1 [file appendix_Q_N.pdf]
