# Supplementary material for: Cell Model Approaches for Predicting the Swelling and Mechanical Properties of Polyelectrolyte Gels
Source: arXiv:1908.10804 source file (2019-11-06)

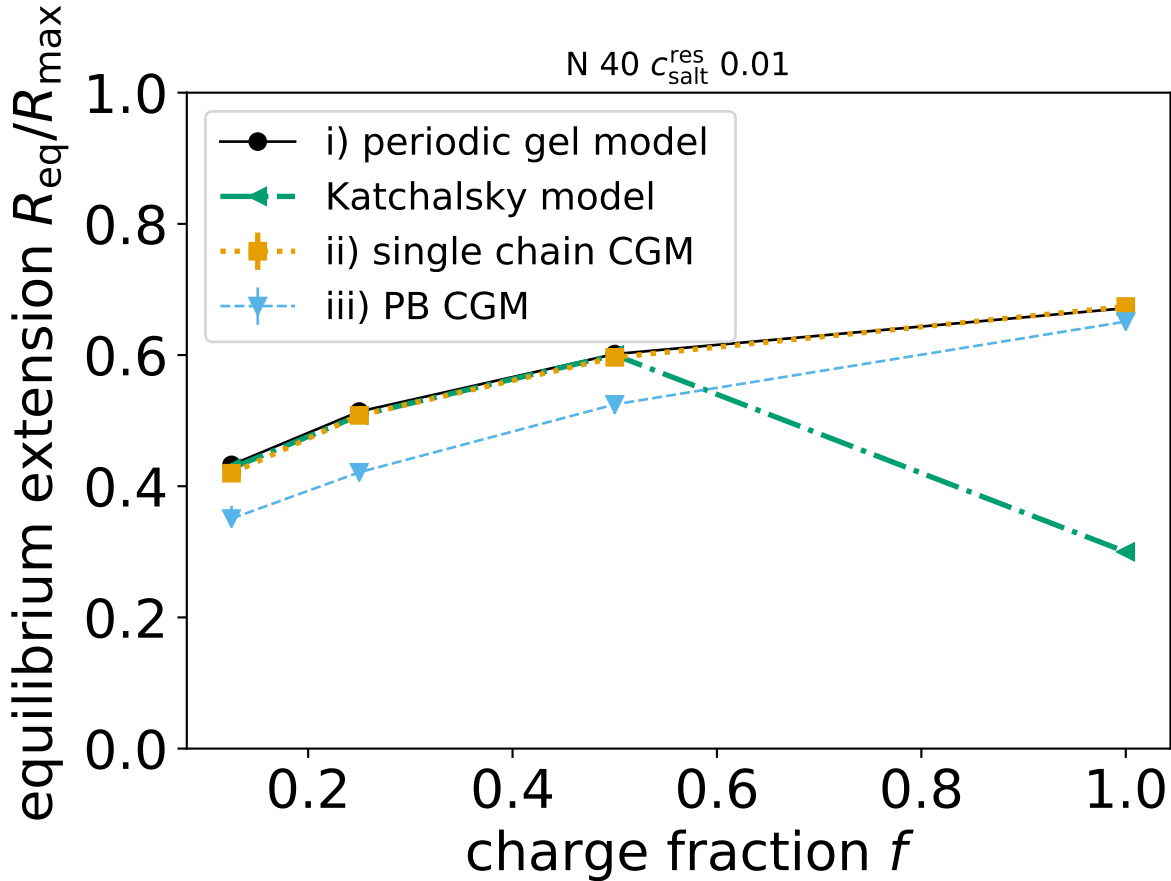

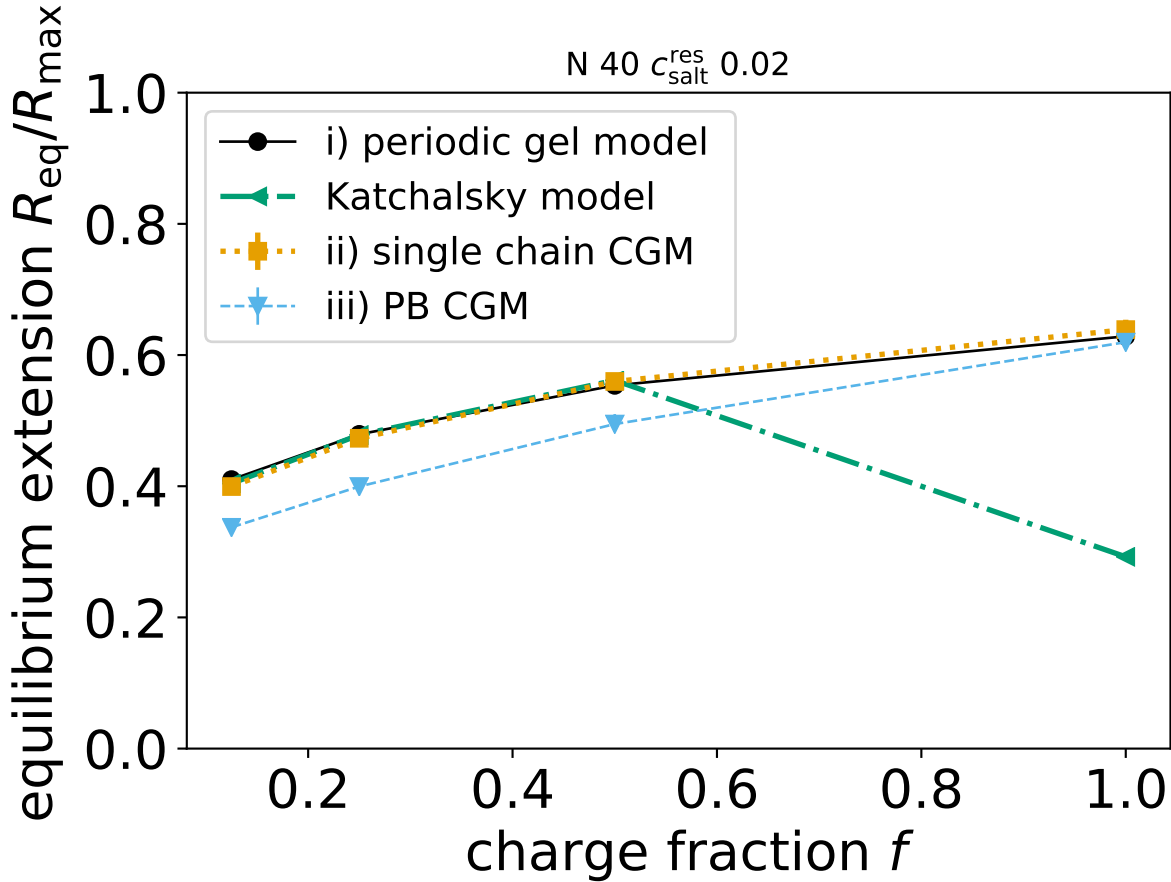

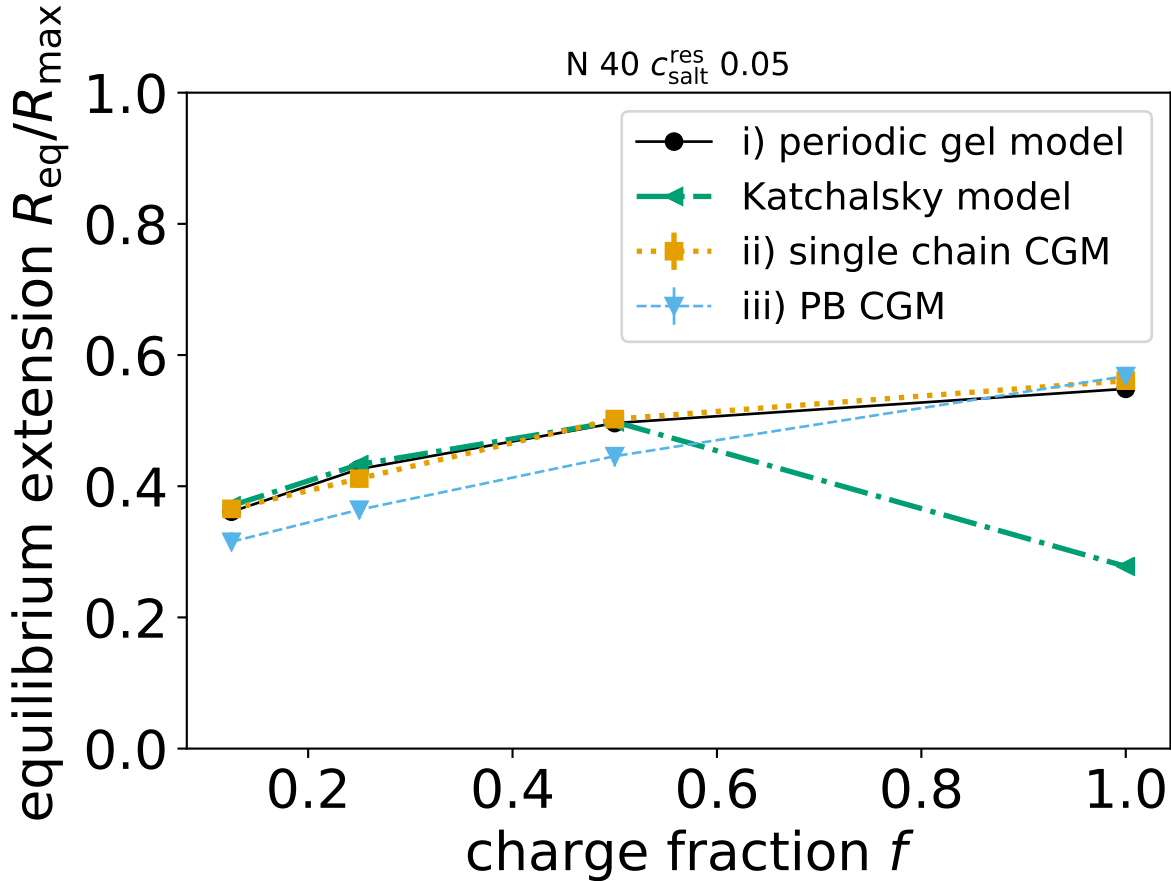

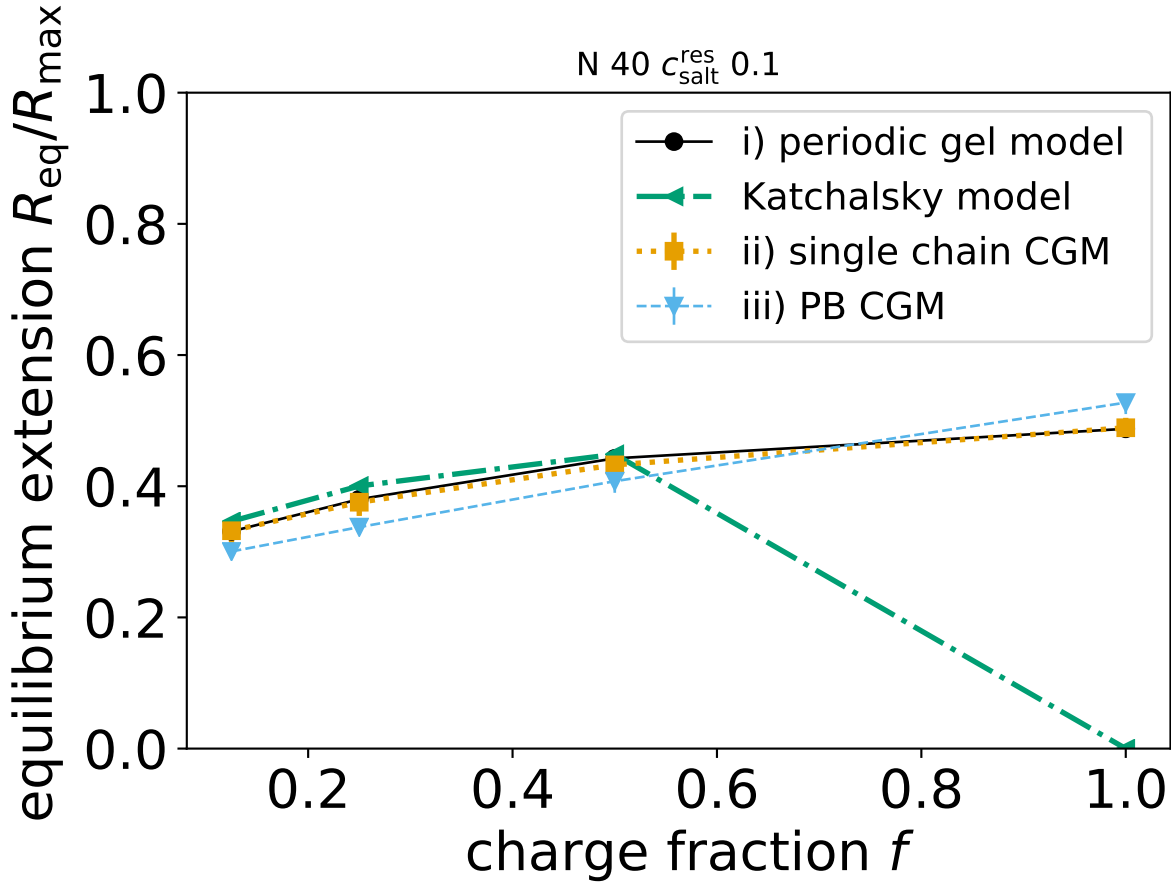

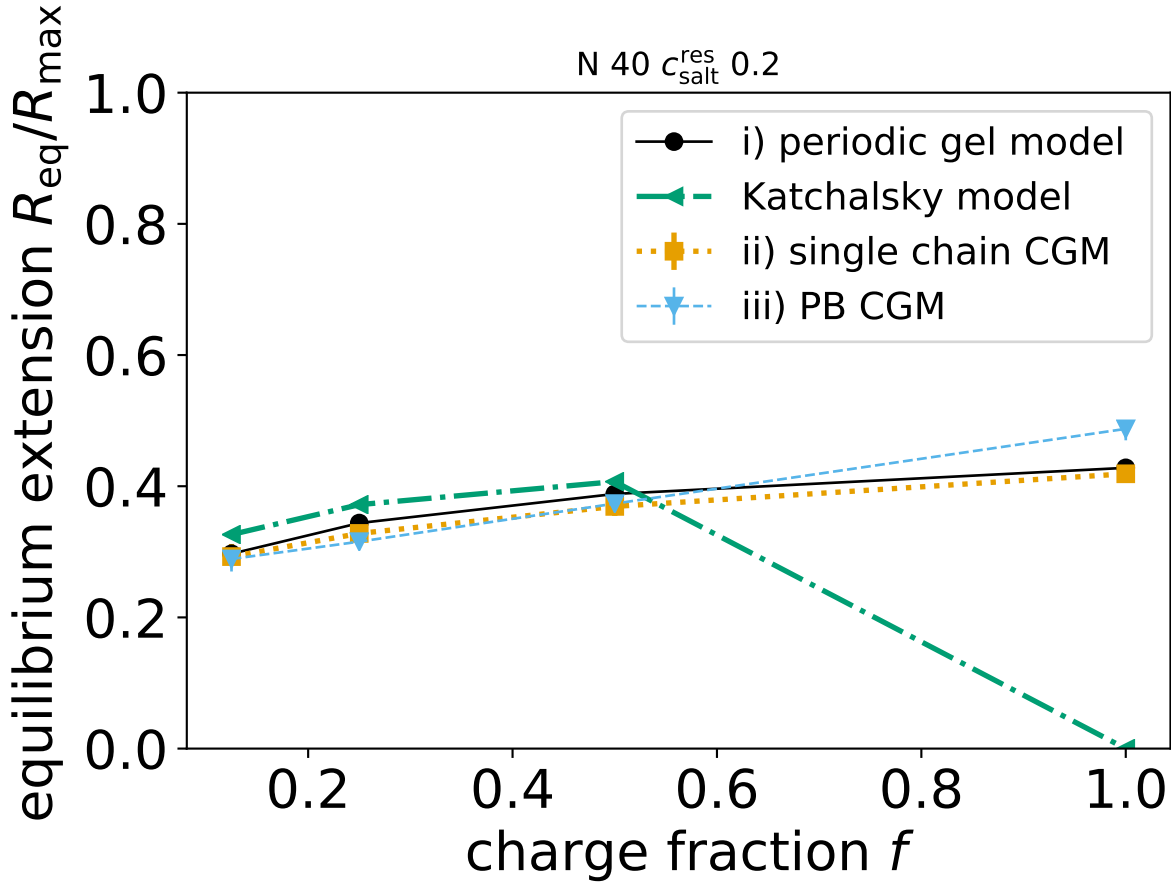

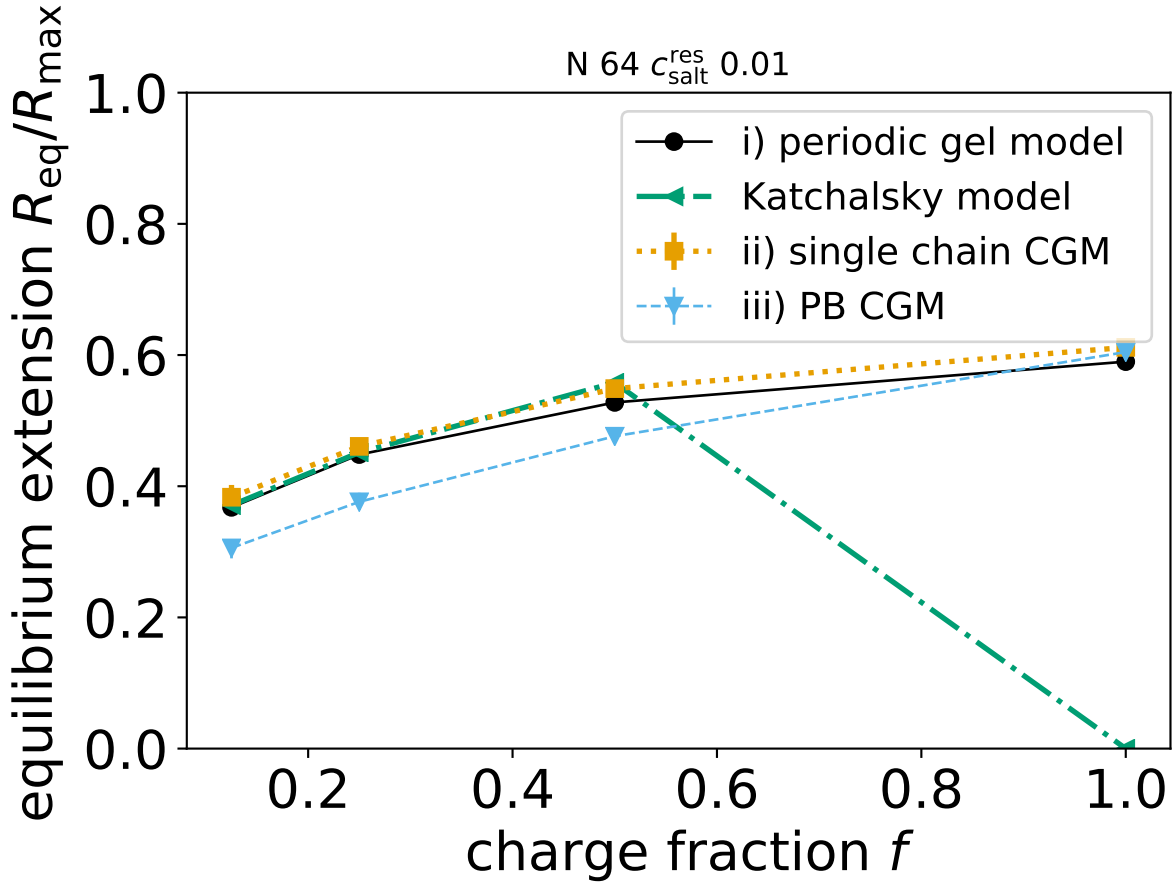

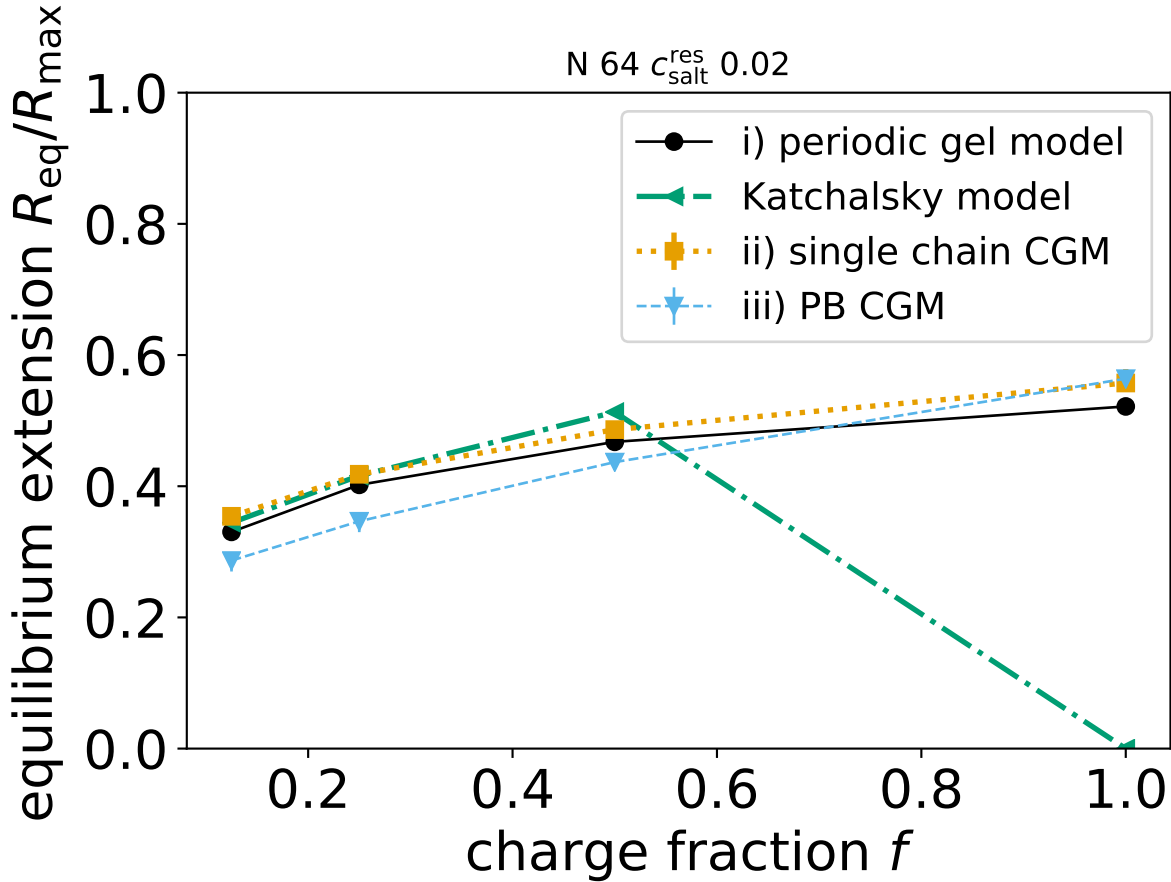

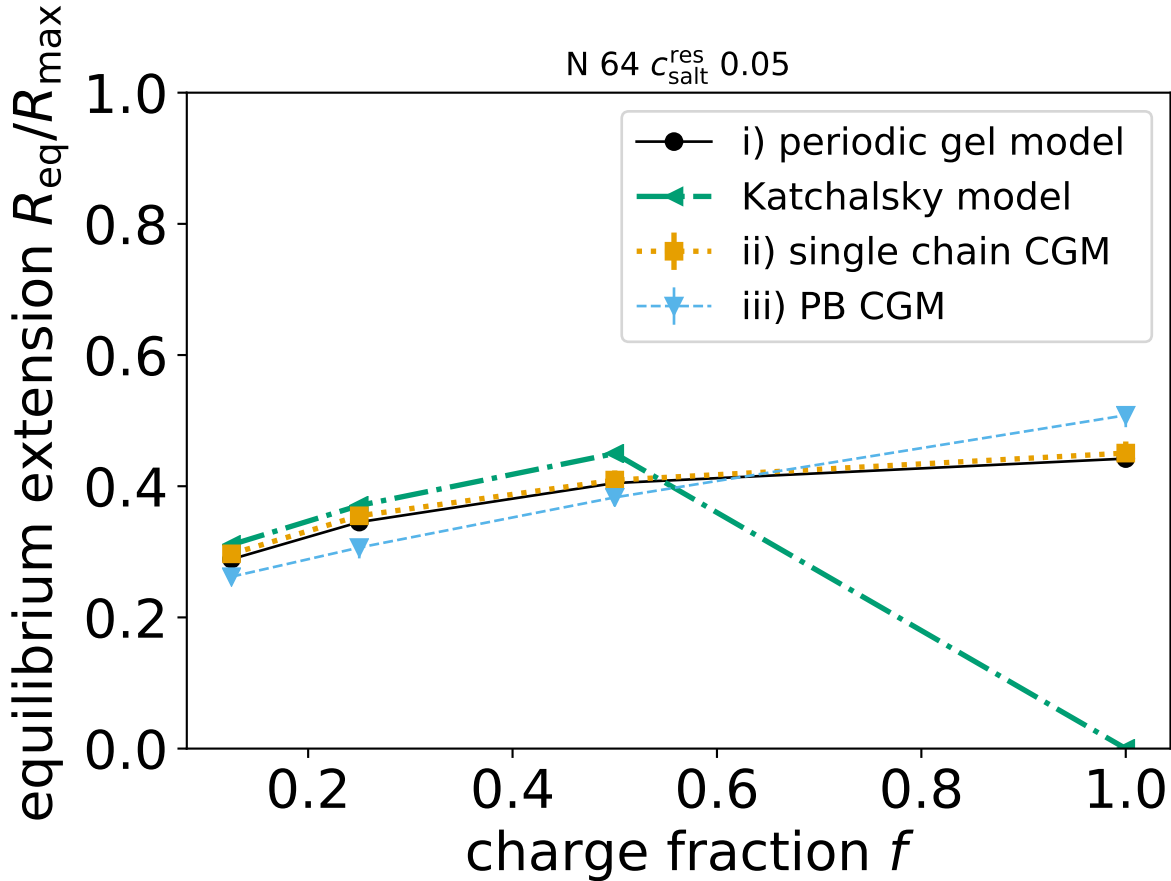



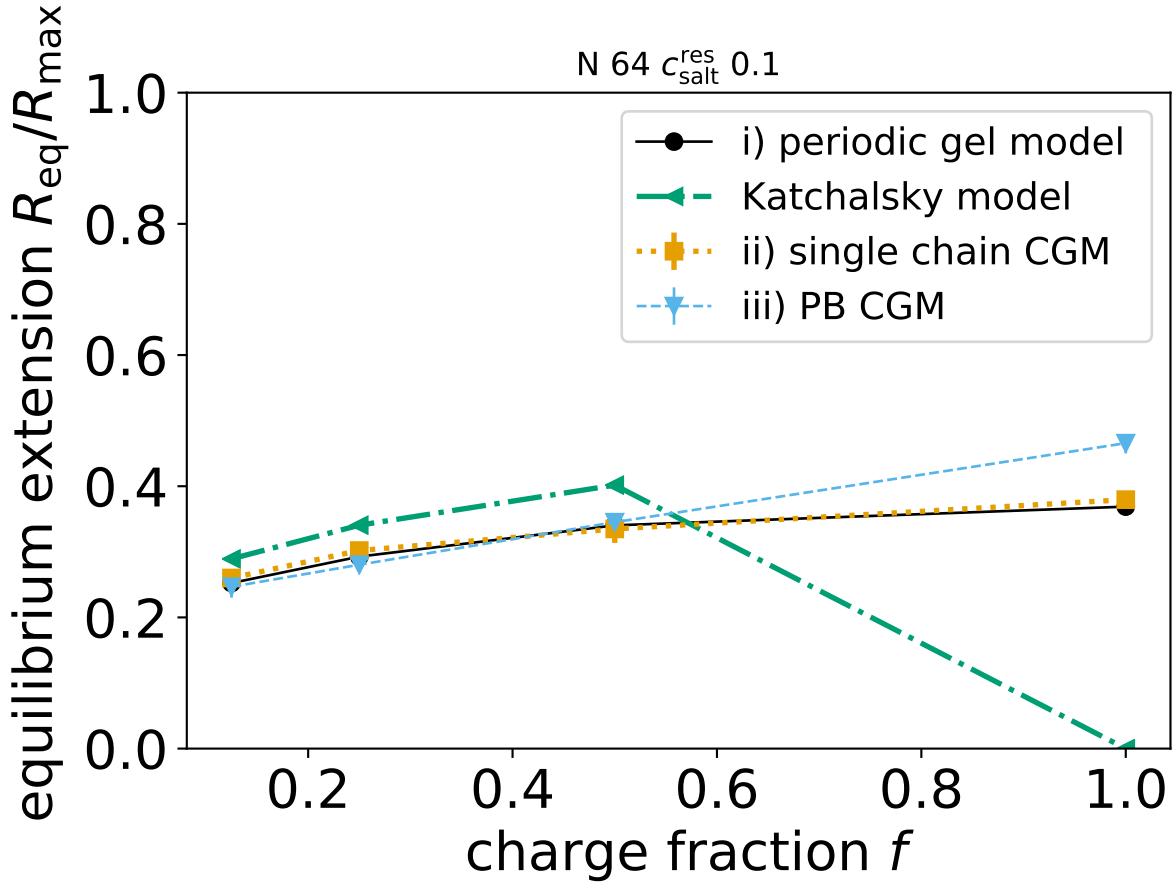

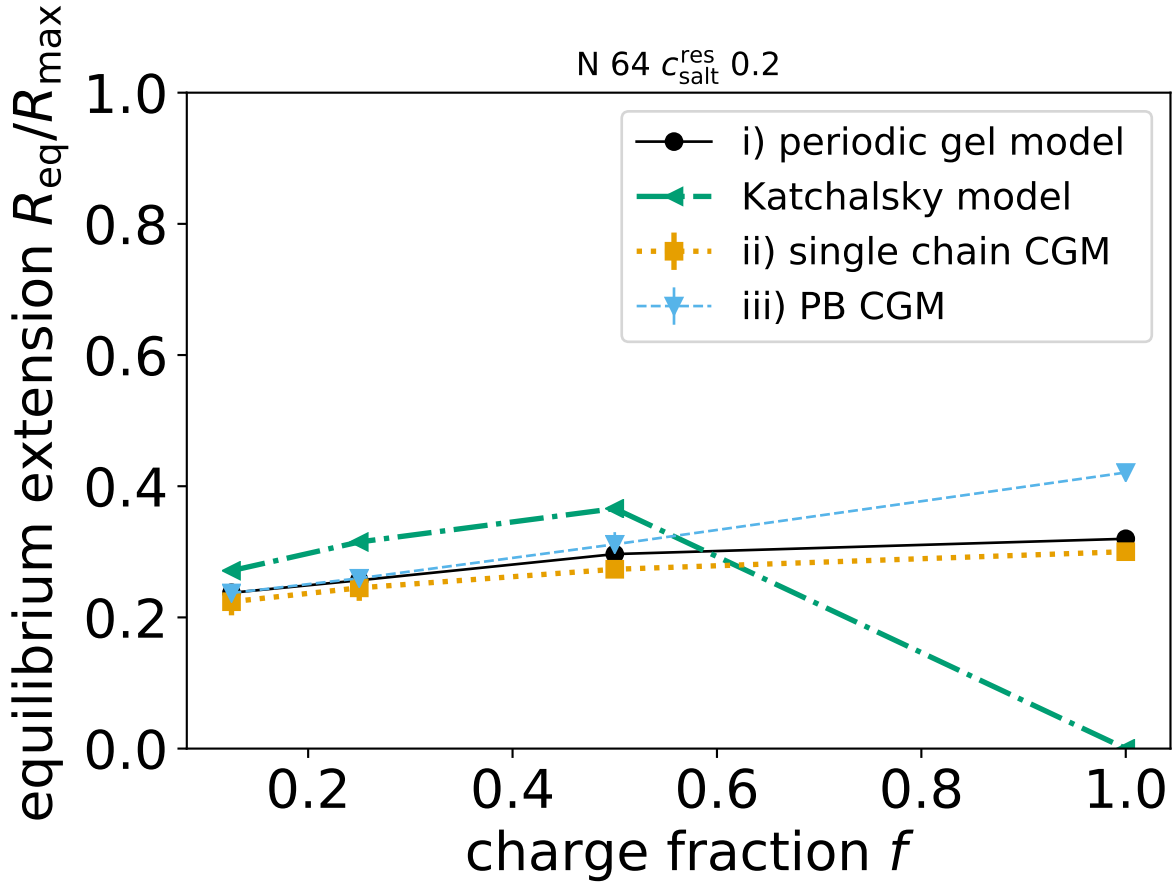

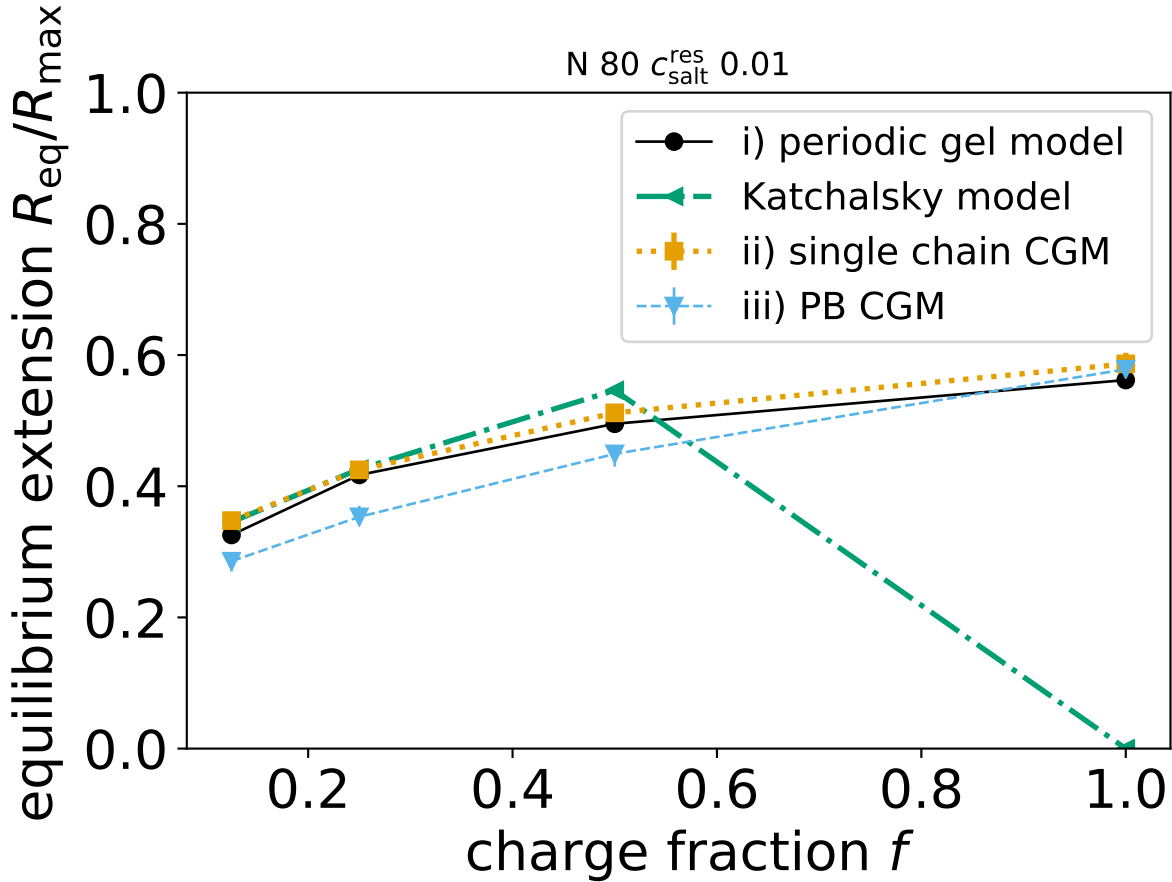

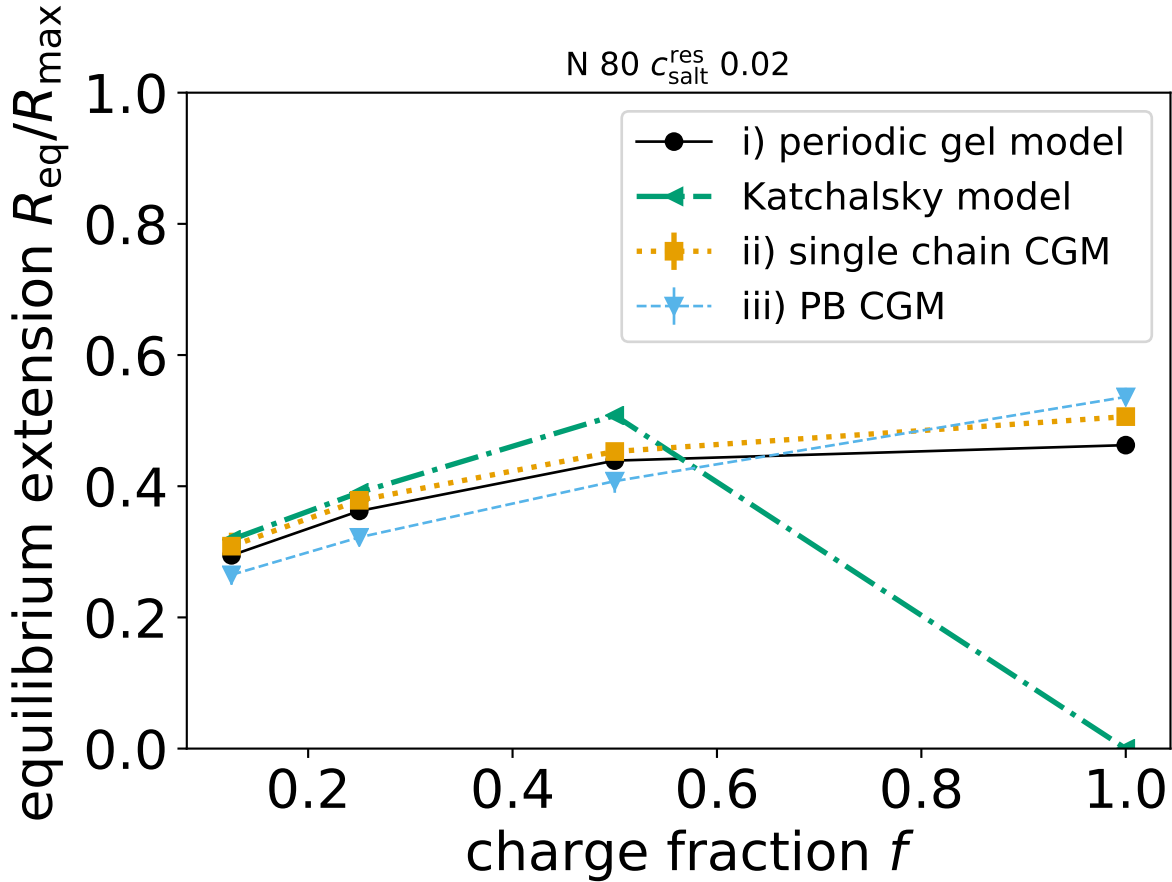

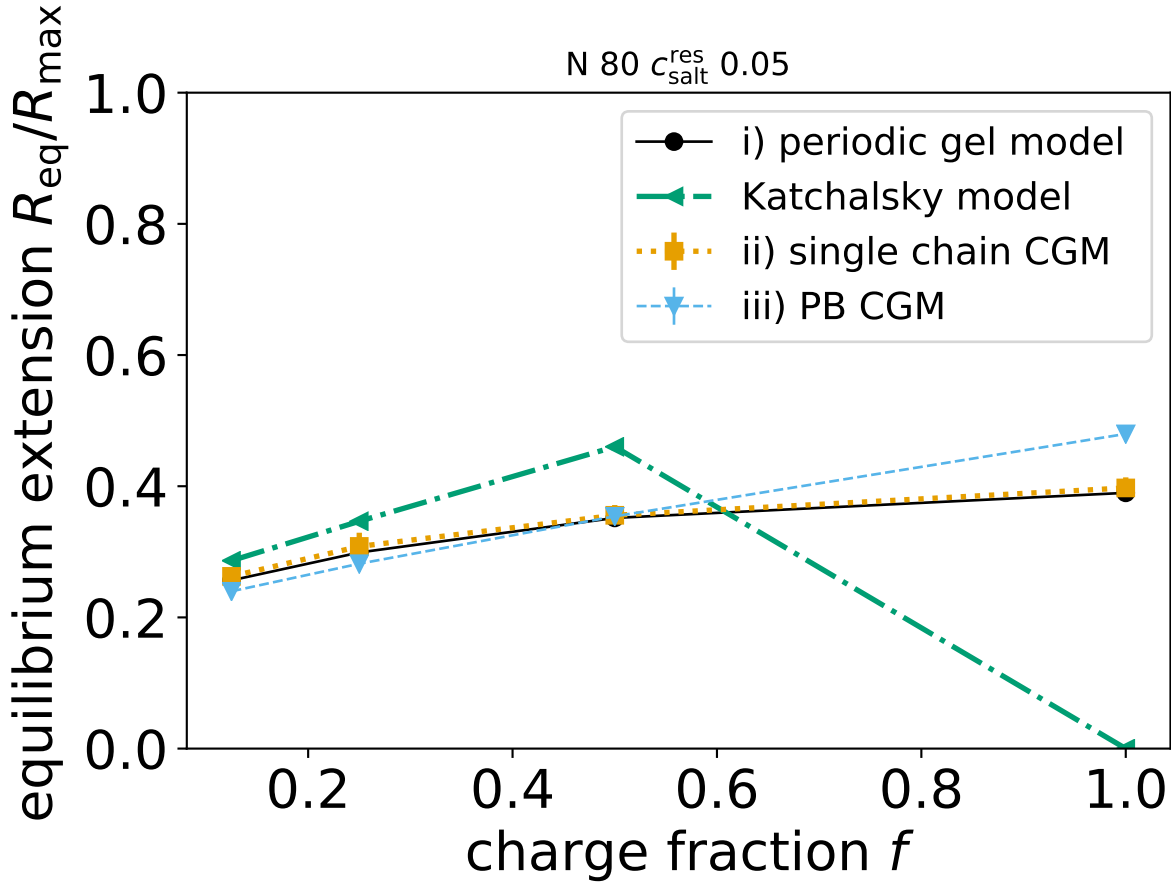

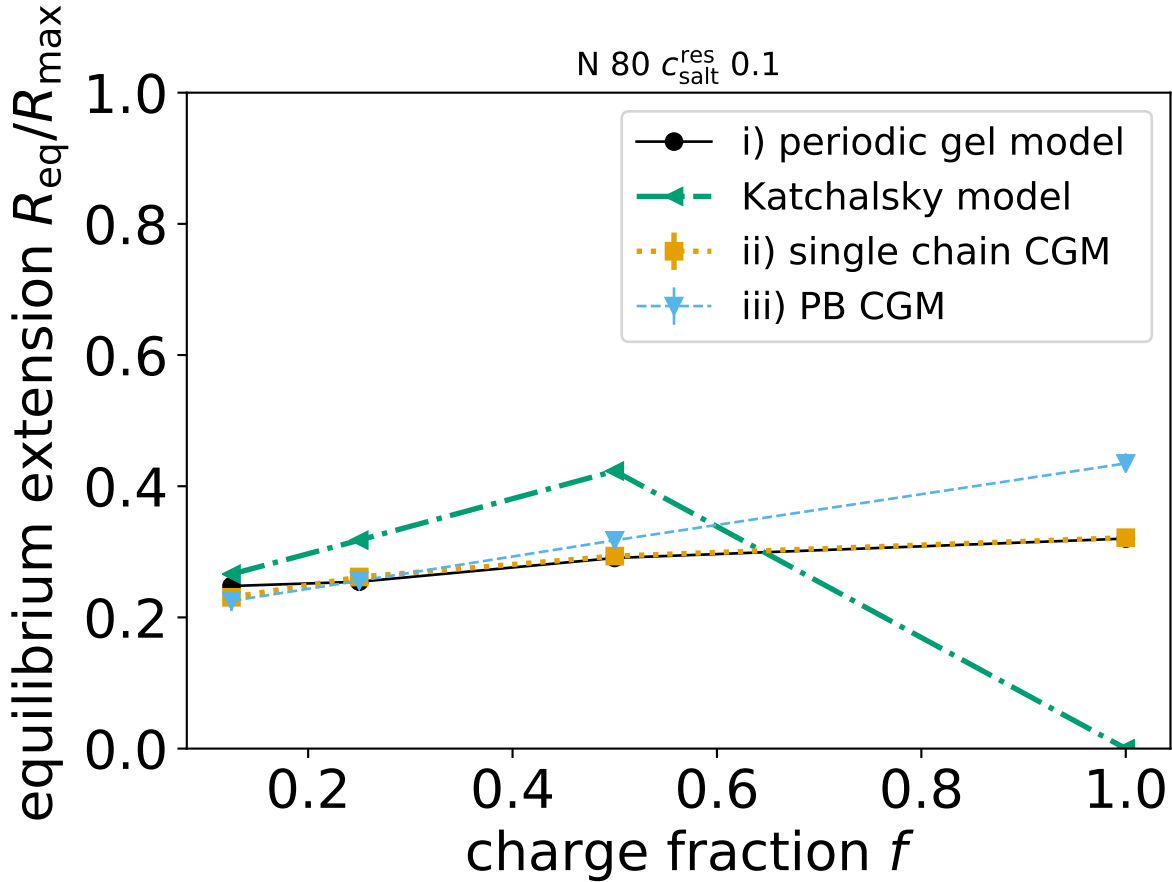

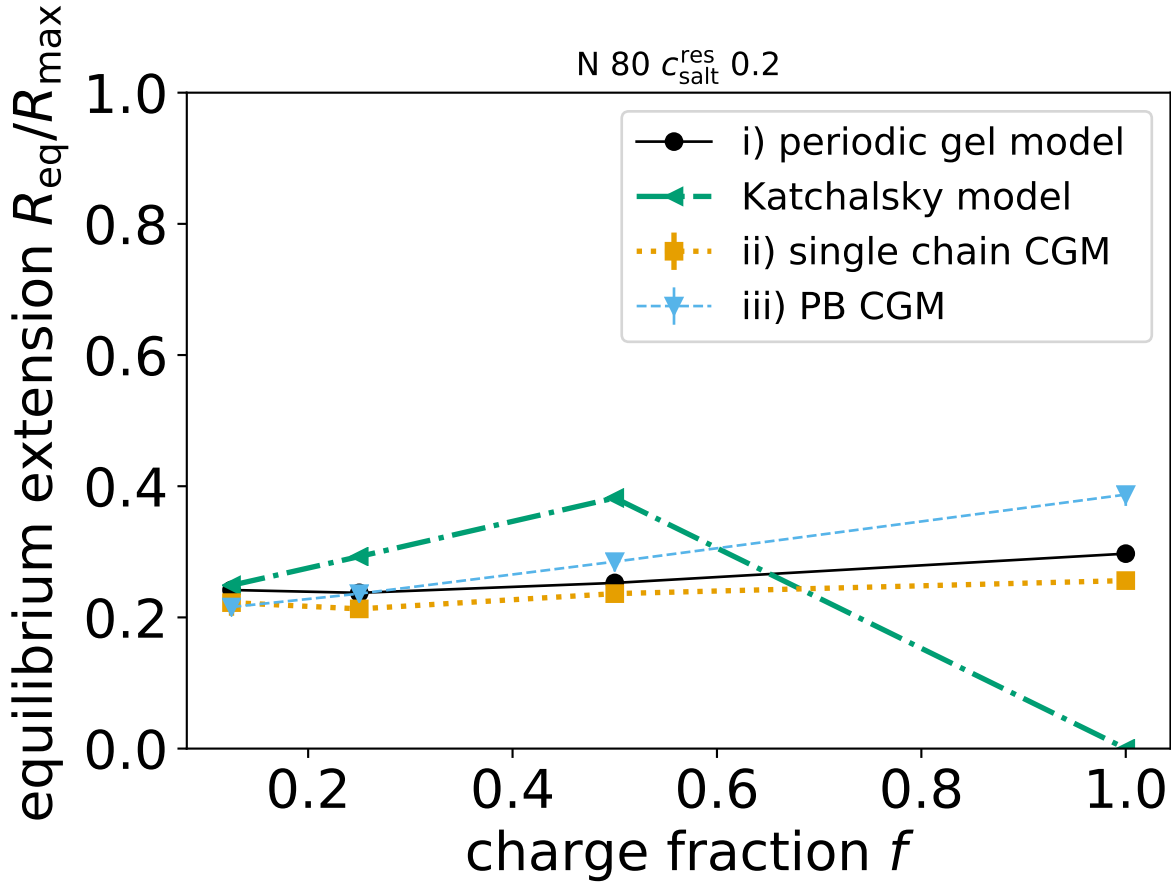

Supplement: Supplementary file 3 [file appendix_Q_f_katchalsky.pdf]
