# Supplementary material for: Cell Model Approaches for Predicting the Swelling and Mechanical Properties of Polyelectrolyte Gels
Source: arXiv:1908.10804 source file (2019-11-06)

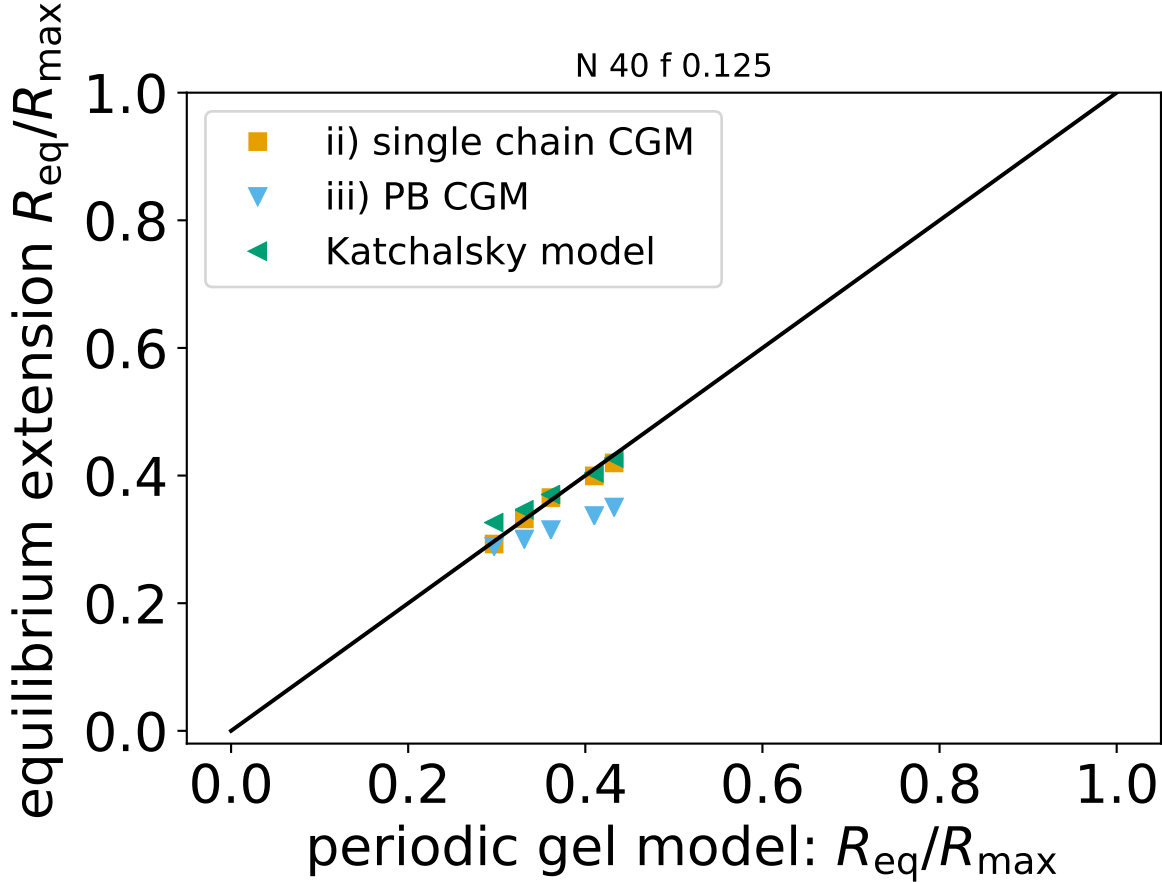

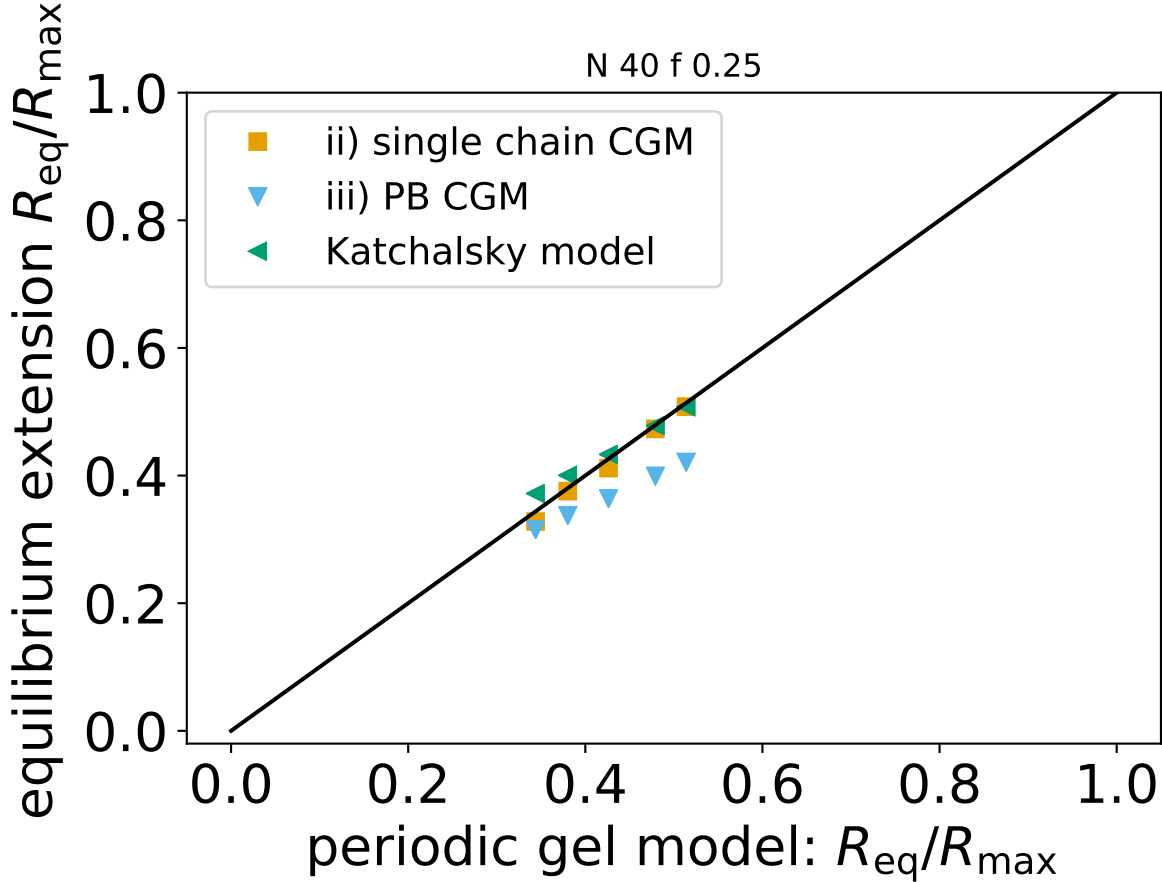

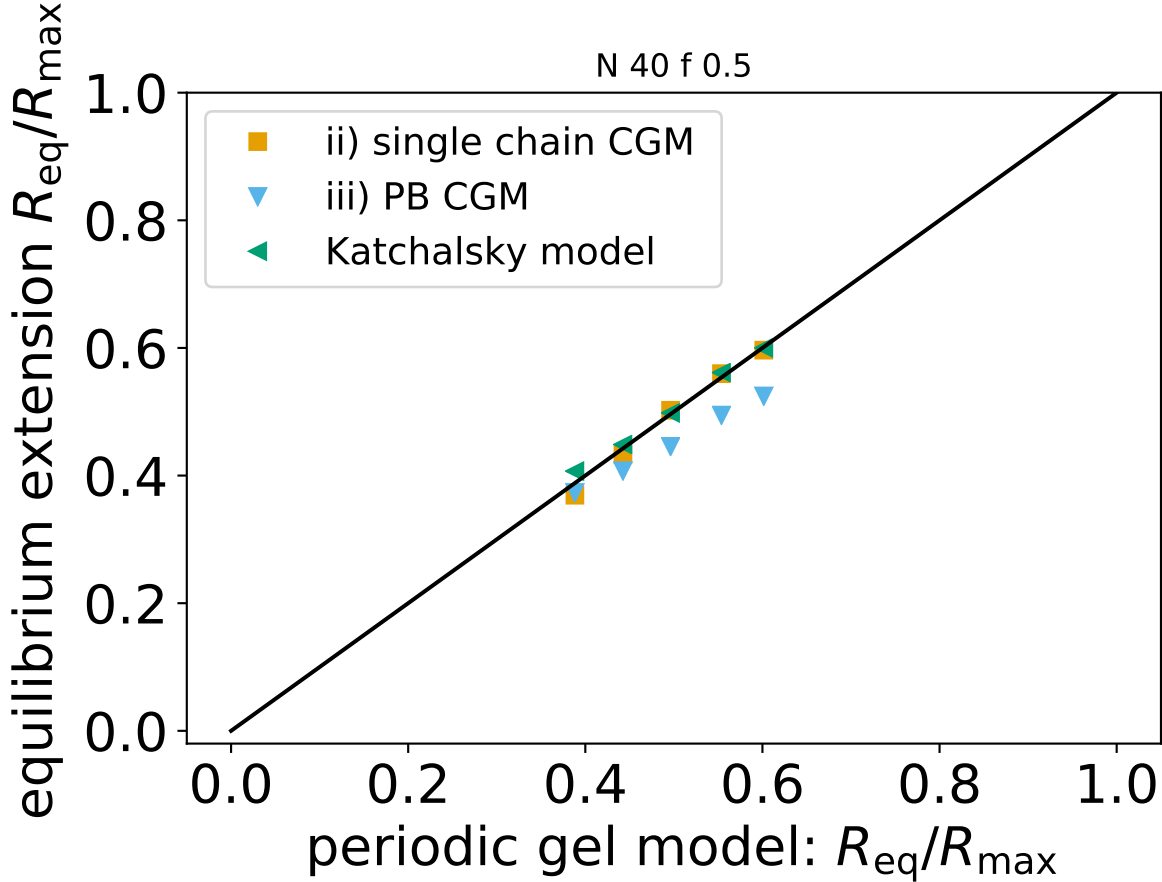

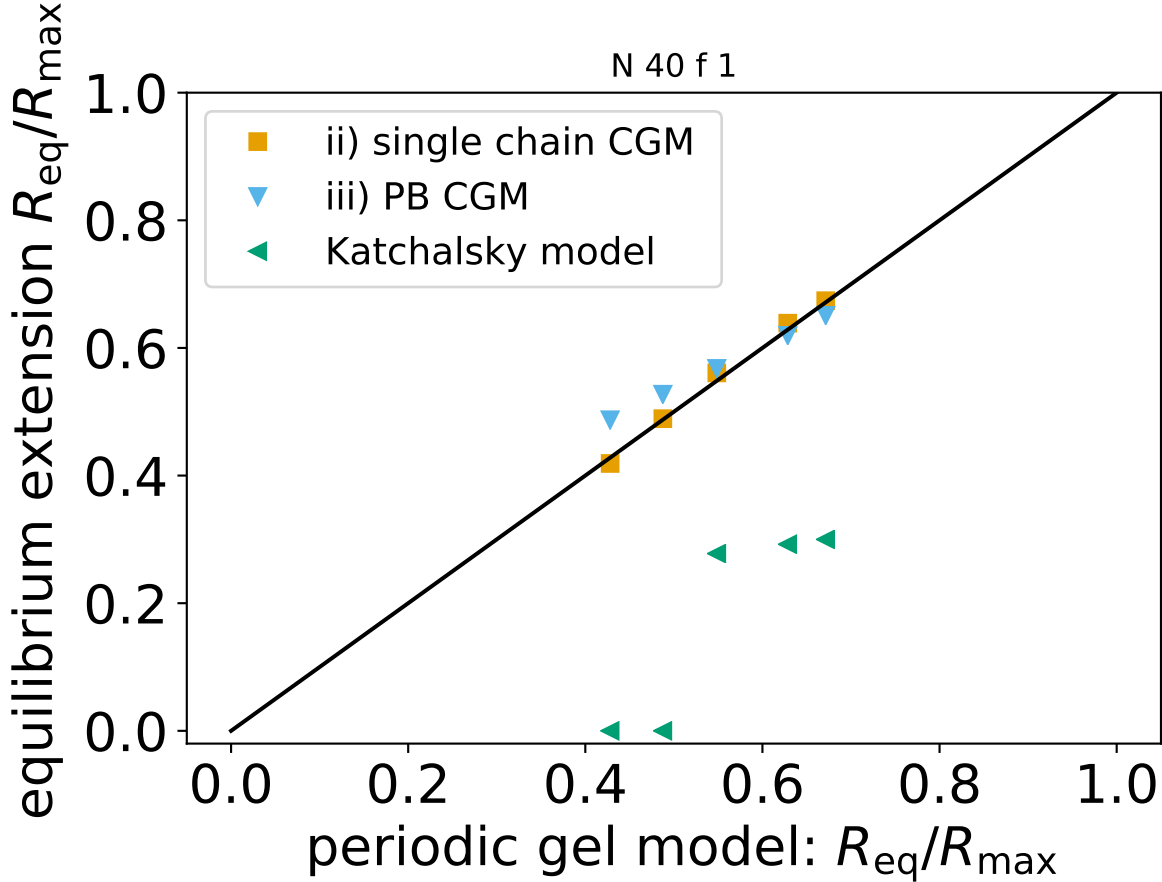

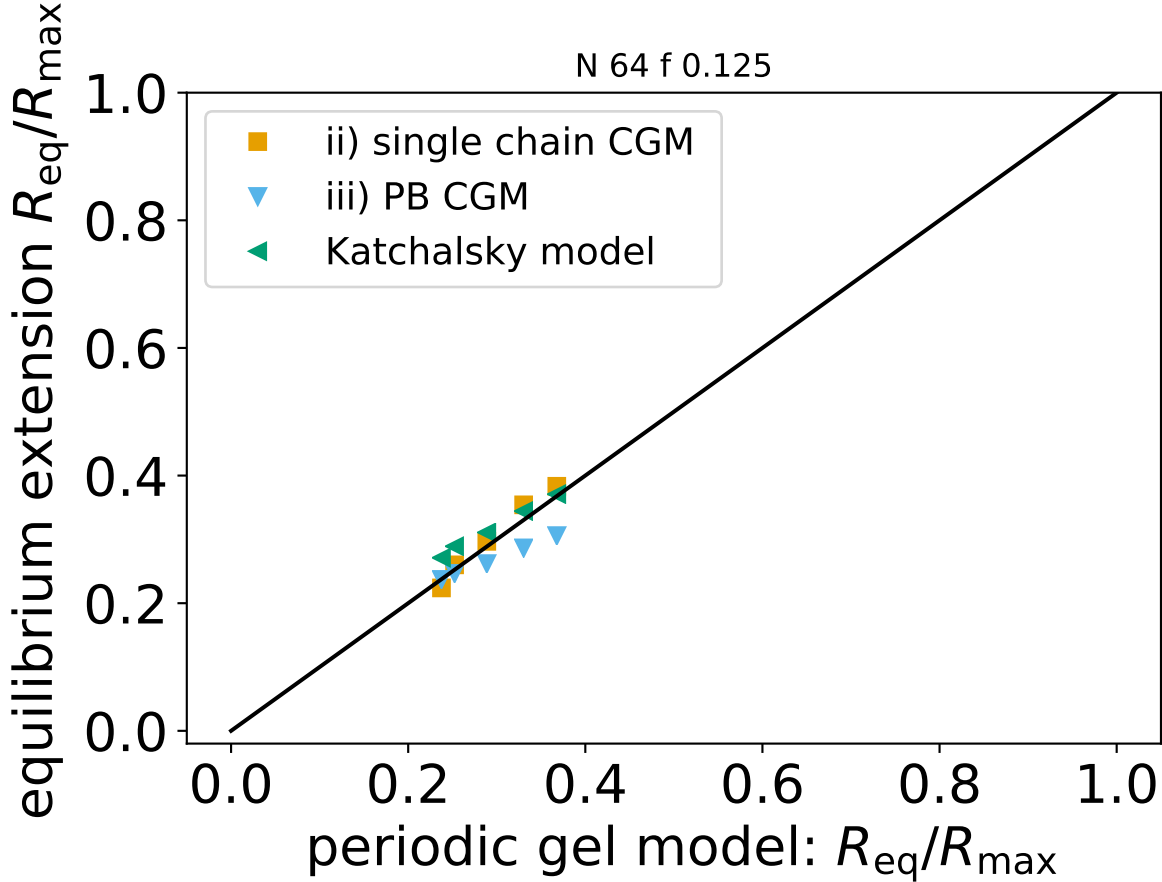

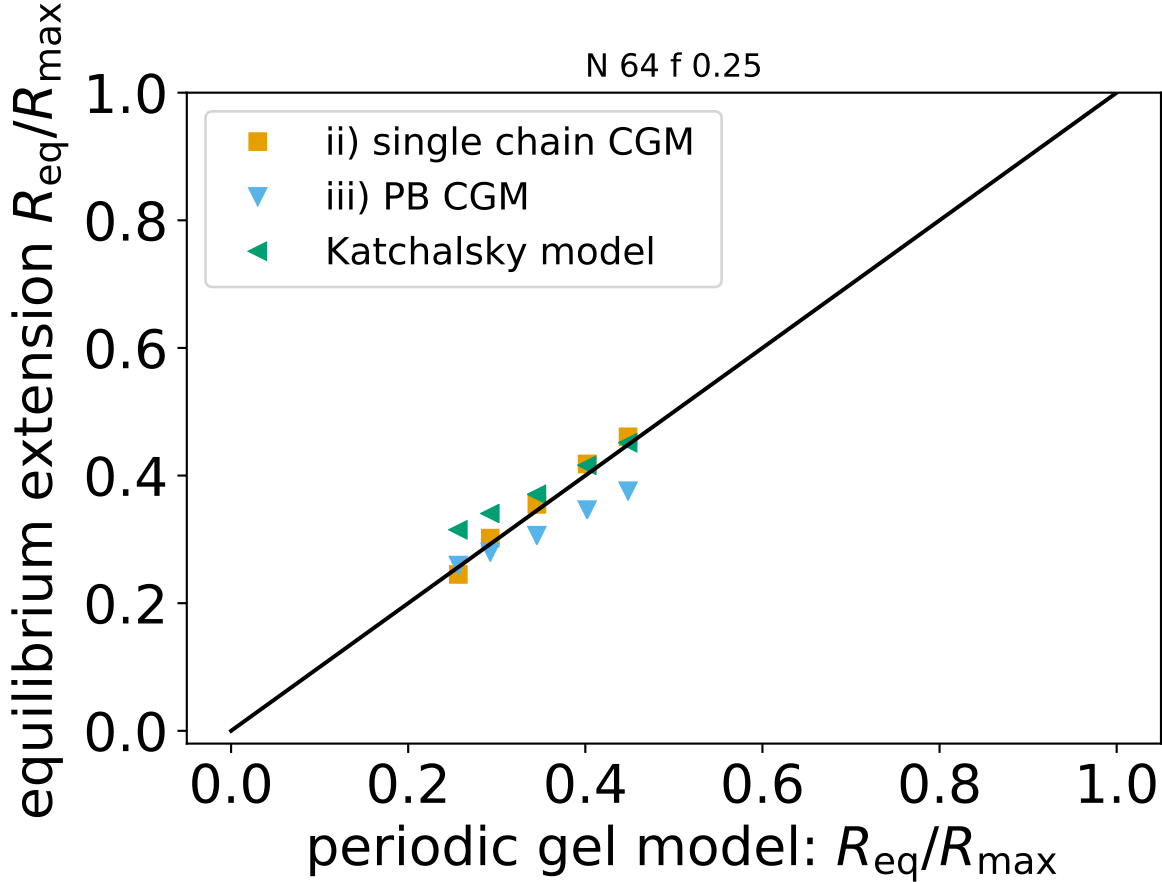

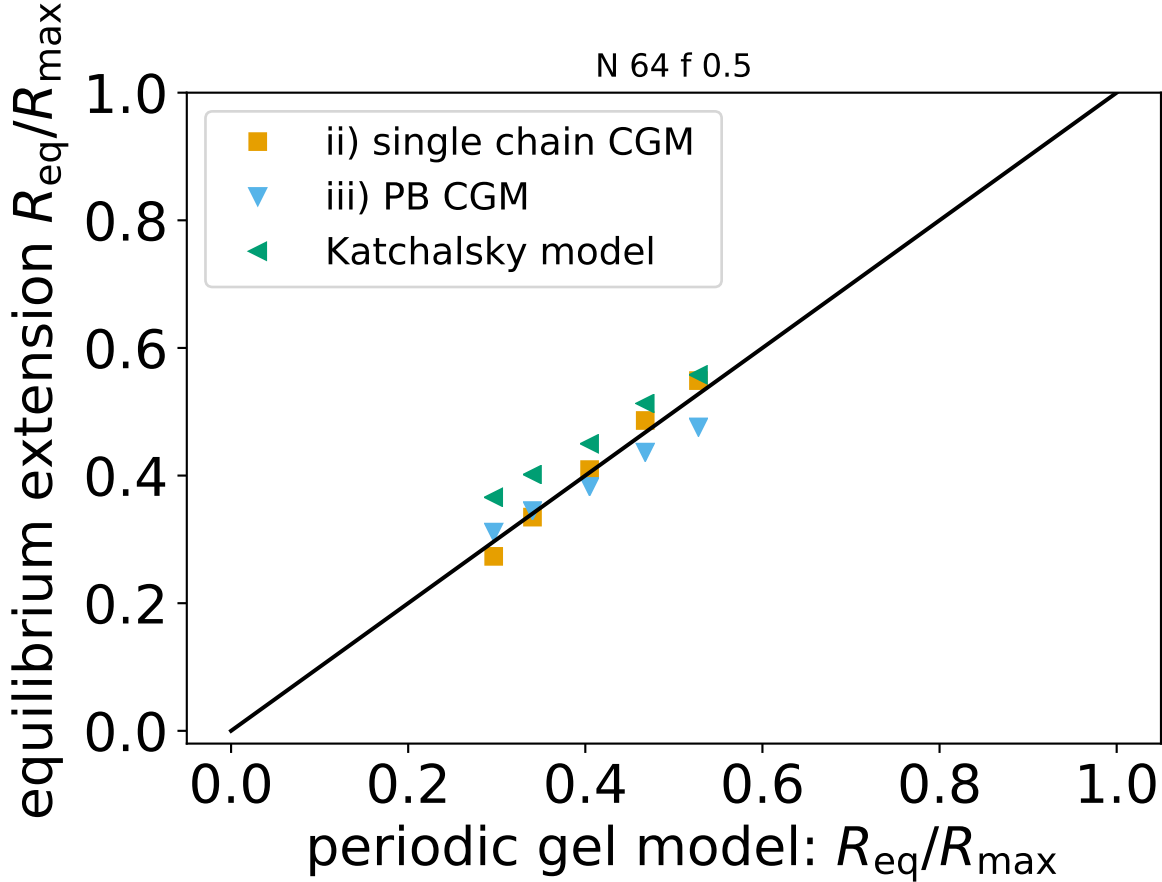

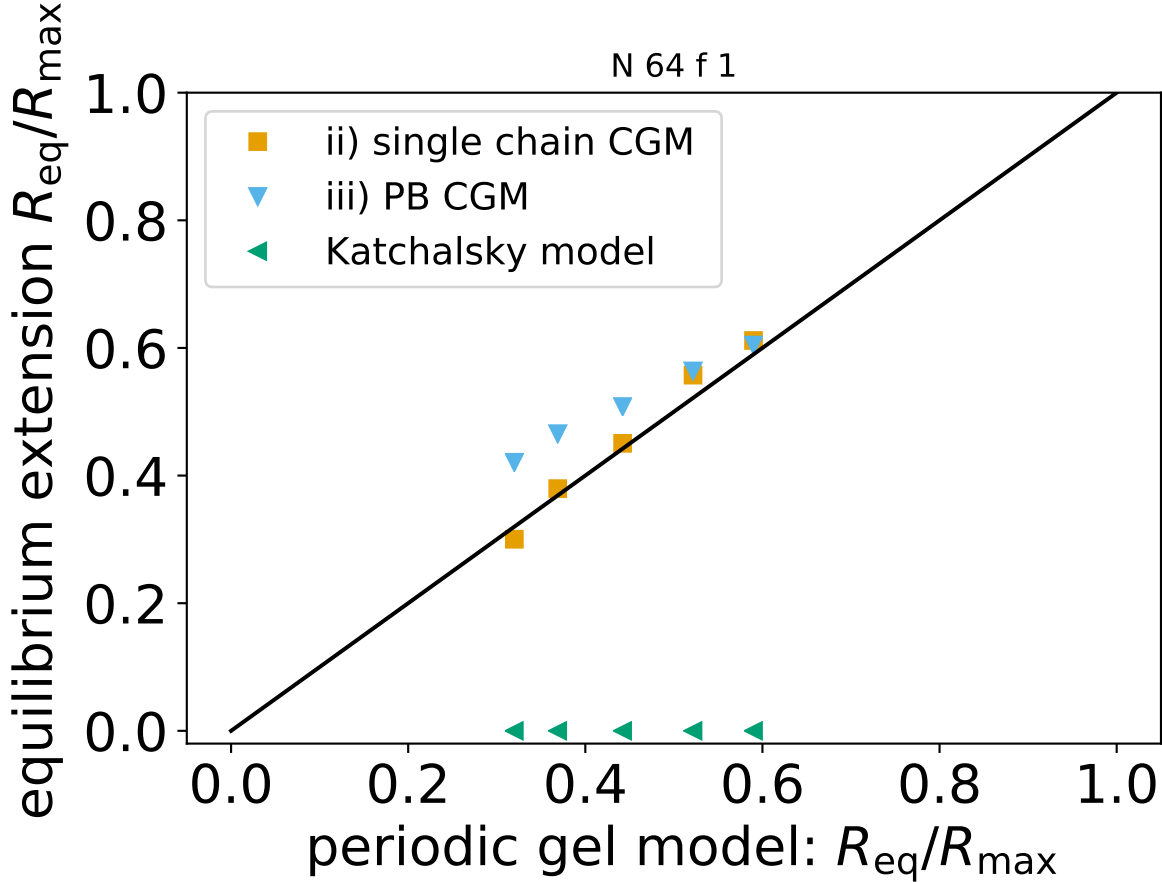



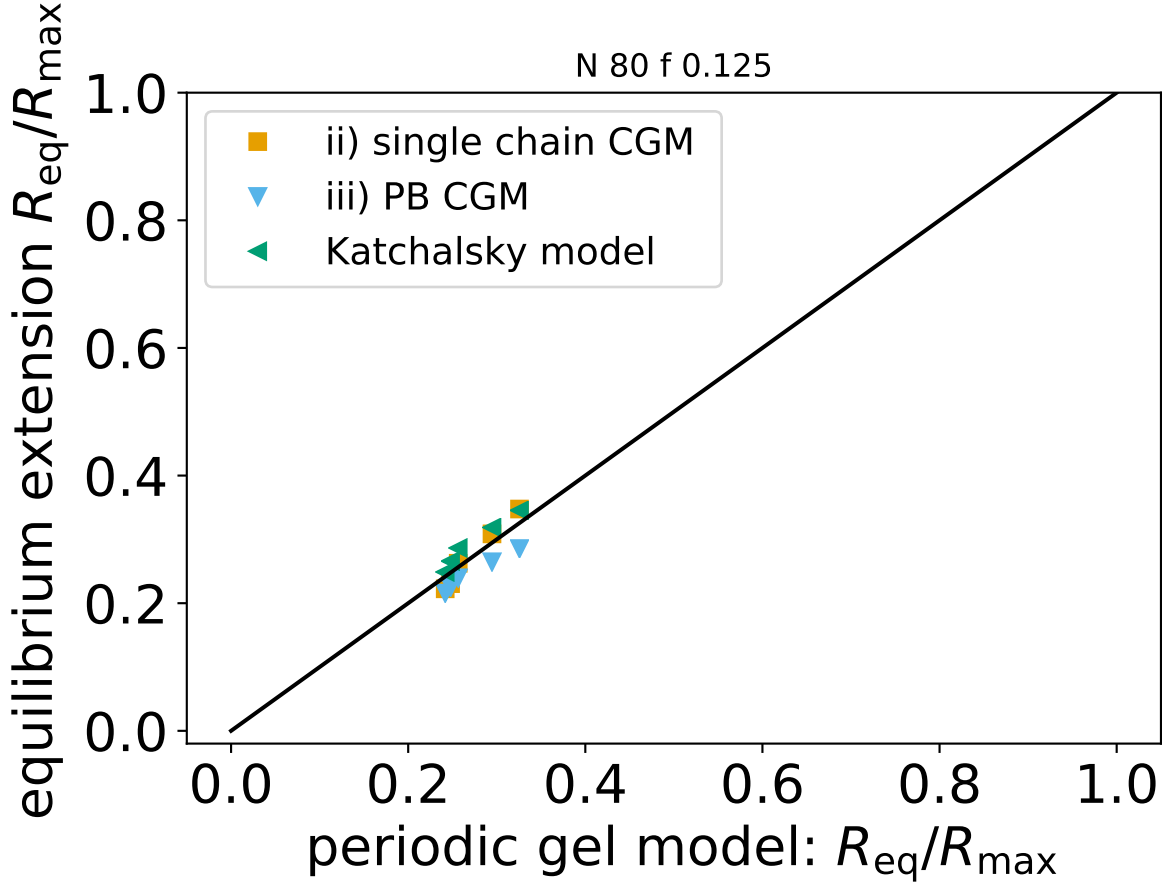

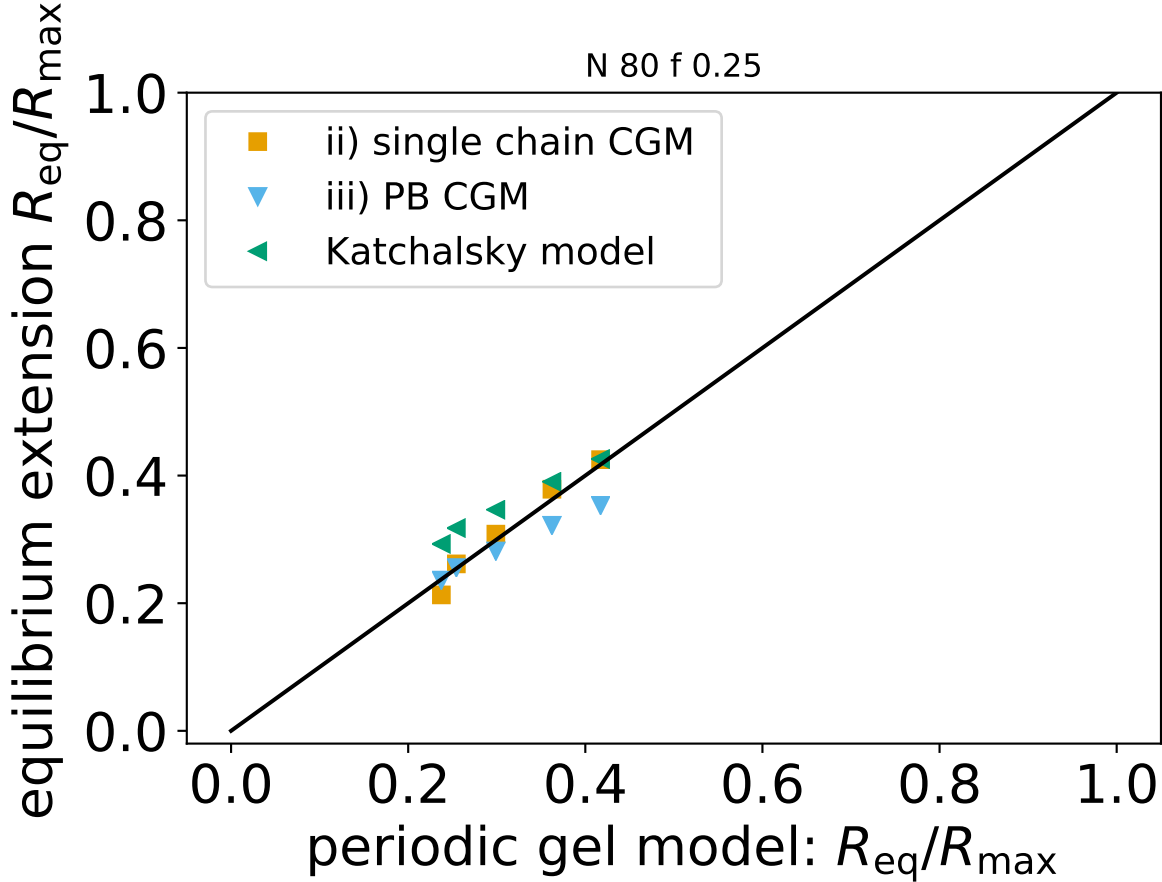

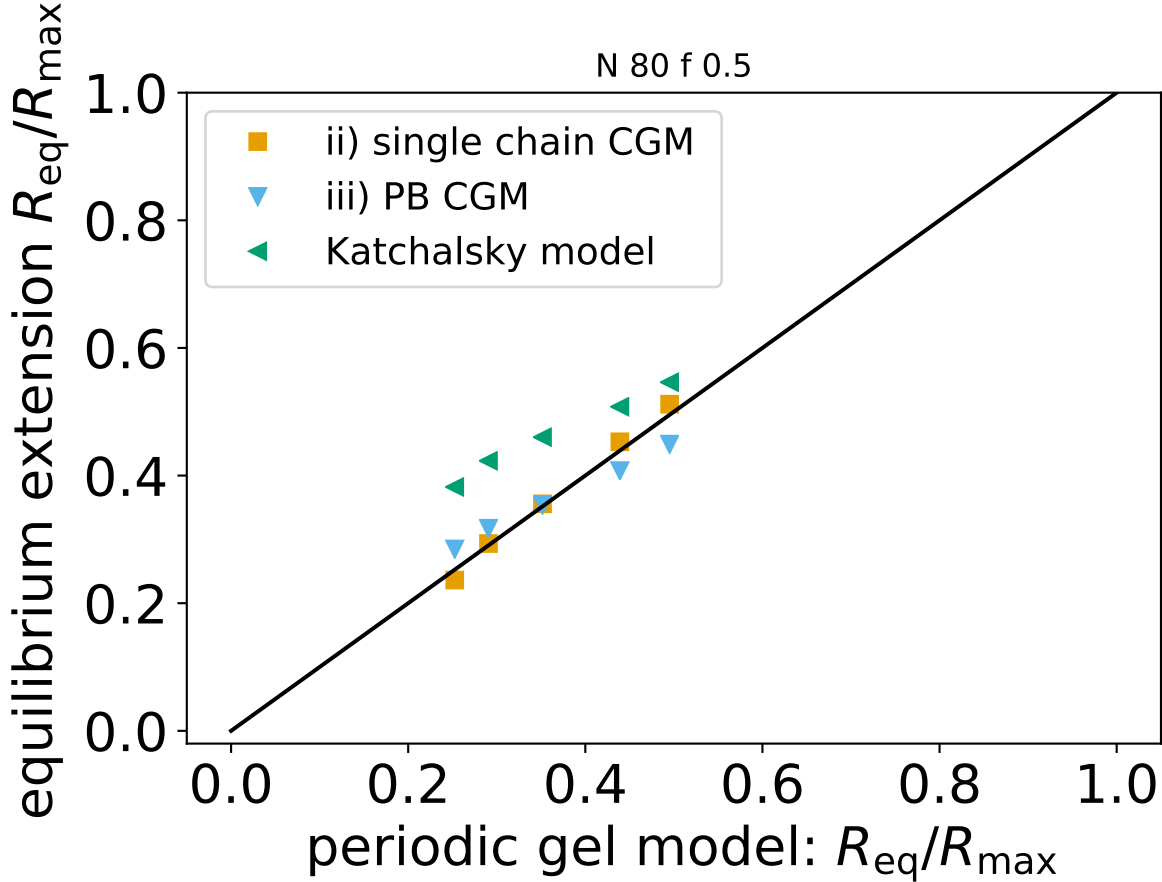

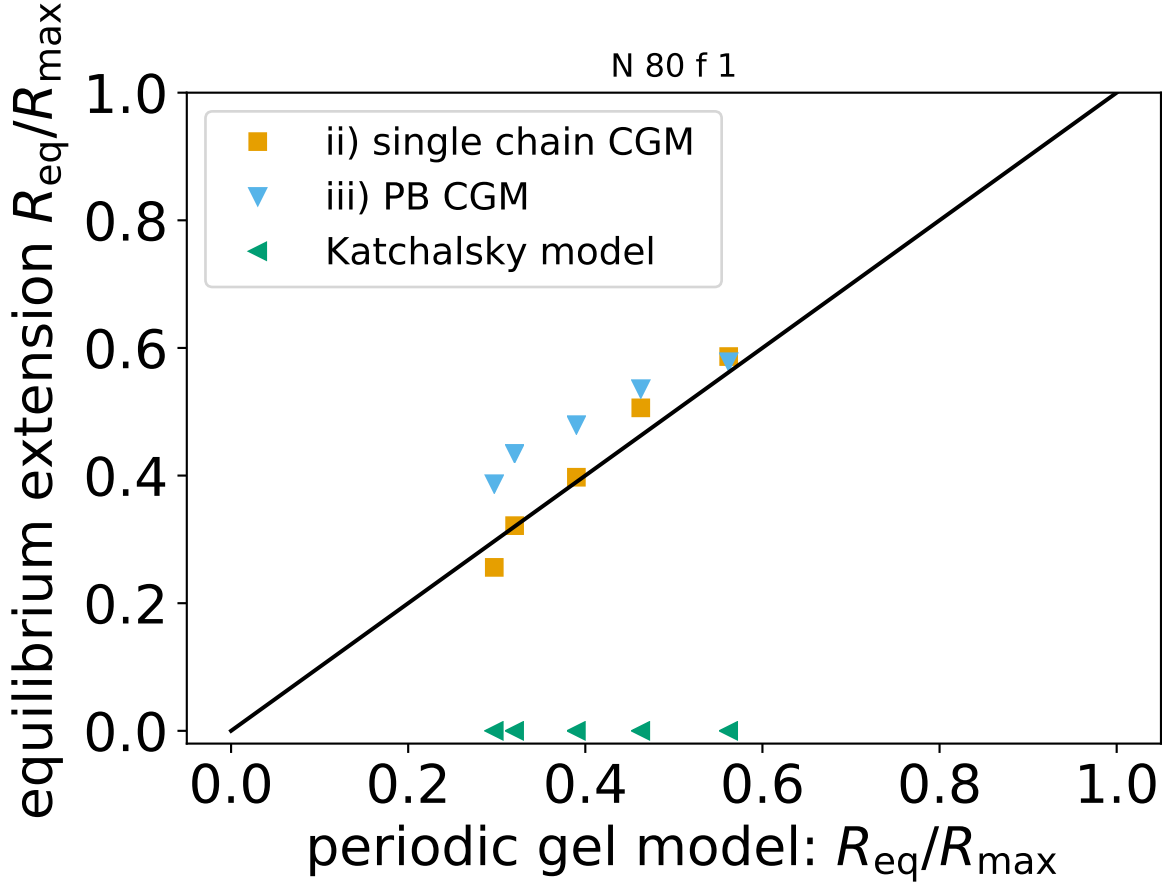

Supplement: Supplementary file 4 [file appendix_correlation_various_cs.pdf]
